# Supplementary material for: MIP-BOOST: Efficient and Effective $L_0$ Feature Selection for Linear Regression
Source: arXiv:1808.02526 ancillary file (2019-09-30)
Supplement: Supplementary file 1 [file Supplement_to_MIP-BOOST_Efficient_and_Effective_L0_Feature_Selection.pdf]

# Supplement to "MIP-BOOST: Efficient and Effective $L_0$ Feature Selection for linear regression"

Ana Kenney*

Dept. of Statistics, Penn State University. University Park PA, USA
and
Francesca Chiaromonte
Inst. of Economics & EMbeDS, Sant'Anna School of Advanced Studies. Pisa, Italy.
and
Giovanni Felici
Istituto di Analisi dei Sistemi ed Informatica, Consiglio Nazionale delle Ricerche. Rome, Italy.

September 30, 2019

**Abstract**

In this document we provide Supplementary Information to the article **MIP-BOOST: Efficient and Effective $L_0$ Feature Selection for Linear Regression**. This includes: (1) detailed pseudocode of each component of MIP-BOOST, (2) correlation structure descriptions through eigenvalue decay, (3) additional results on the effects of whitening, (4) full results comparing statistical quality from our simulation study which were not included in the main text due to space limitations, (5) additional figures illustrating the MIP-BOOST speedup, and (6) a proof sketch for convergence of our Bisection with Feelers algorithm. Code utilized for the implementation of the proposed methodology and to generate simulated data is available upon request.

*We thank Matthew Reimherr for useful discussions and comments. This work was partially funded by the NIH B2D2K training grant and the Huck Institutes of the Life Sciences of Penn State, and by NSF grant DMS-1407639. Computation was performed on the Institute for CyberScience Advanced CyberInfrastructure (ICS-ACI; Penn State University).

# Contents

**1 Pseudocode for MIP-BOOST** **3**

**2 Correlation Structures** **4**

**3 Whitening Comparisons** **5**

**4 Full Results for Statistical Quality** **8**

4.1 Scenarios with $p = 100$ and constant $\boldsymbol{\beta}$ coefficients . . . . . . . . . . . . . . . 8

4.2 Scenarios with $p = 100$ and varying $\boldsymbol{\beta}$ coefficients . . . . . . . . . . . . . . . 13

4.3 Scenarios with $p = 1000$ and constant $\boldsymbol{\beta}$ coefficients . . . . . . . . . . . . . . 18

4.4 Scenarios with $p = 1000$ and varying $\boldsymbol{\beta}$ coefficients . . . . . . . . . . . . . . 23

4.5 Sparser scenarios with $p = 100$ . . . . . . . . . . . . . . . . . . . . . . . . . . . 28

**5 Additional Results for the Computational Burden** **29**

**6 Bisection with Feelers Convergence Proof Sketch** **31**

# 1 Pseudocode for MIP-BOOST

**Algorithm 1:** Bisection with Feelers (BF) and LASSO Search Rule

**input** : Initial lower bound $a_0$ and upper bound $c_0$ (where $c_0$ is the number of variables produced through LASSO), maximum number of iterations *itermax*, threshold of improvement $\delta$. and feeler search length $l_f$

**output** : Selected sparsity bound $\hat{k}_0$

Set $a = a_0$ and $c = c_0$; **for** $i = 1$ **to** *itermax* **do**
    **while** $a \neq b$ **do**
        Bisect interval at $b = \text{floor}(\frac{a+c}{2})$
        Solve for $M_a$, $M_b$, and $M_c$
        Calculate $\Delta f(a, b)$ and $\Delta f(b, c)$
        **if** $\Delta f(b, c) > \delta$ **and** $\Delta f(a, b) > -\delta$ **then**
            Search interval $[b, c]$ by setting $a = b$
        **else**
            Search interval $[a, b]$ by setting $c = b$
        **end**
    **end**
    Now the interval is $[a, b, c]$ where $b = a$ and $c = a + 1$
    **if** $\Delta f(a, c) > \delta$ **then**
        Set $\hat{k}_0 = c$
    **else**
        Set $\hat{k}_0 = a$
    **end**
    Solve for the two feelers $M_{\hat{k}_0 - l_f}$ and $M_{\hat{k}_0 + l_f}$
    Calculate $\Delta f(\hat{k}_0 - l_f, \hat{k}_0)$ and $\Delta f(\hat{k}_0, \hat{k}_0 + l_f)$
    **if** $\Delta f(\hat{k}_0 - l_f, \hat{k}_0) > \delta$ **and** $\Delta f(\hat{k}_0, \hat{k}_0 + l_f) < \delta$ **then**
        break
    **else if** $\Delta f(\hat{k}_0, \hat{k}_0 + l_f) > \delta$ **then**
        Too sparse, set $a = \hat{k}_0 + l_f$ and $c = c_0$
    **else**
        Stuck in the tail, set $a = 1$ and $c = \hat{k}_0 - l_f$
    **end**
**end**

**Algorithm 2:** Integrated Cross-Validation (ICV), Warm Starts, and Surrogate Lower Bounds (SLB)

**input** : Sparsity bound $k$, cross-validation folds $\mathcal{F}_v$ where $v = 1, ..., V$, relaxation parameter $\tilde{\mathcal{M}}$, maximum computing time *maxtime* before SLB, total computing time *totaltime*, true gap threshold $\epsilon_G$, and surrogate gap threshold $\epsilon_{FS^+}$

```
for v = 1 to V do
    Take m_i = M̃ I(i ∈ F_v) for i = 1, .., n
    if v = 1 then
        Run forward selection on left-in folds at k to get z_FS and β_FS
        Relax constraints by m_i and solve for M_k starting from z_FS and β_FS
        if Computing time ≥ maxtime and MIP gap ≥ ε_G then
            Run forward selection on left-in folds at k + 1 to get E_FS+
            while Computing time ≥ totaltime or surrogate MIP gap ≤ ε_FS+ do
                Continue solving
            end
        end
    else
        Relax constraints by m_i and solve for M_k starting from previous MIP solution
        if surrogate triggered previously or Computing time ≥ maxtime then
            while Computing time ≥ totaltime or surrogate MIP gap ≤ ε_FS+ do
                Continue solving
            end
        end
    end
end
```

**Algorithm 3:** Whitening

**input** : Data matrix $\mathbf{X}$ and response vector $\boldsymbol{Y}$

1. Estimate $\boldsymbol{\Sigma}^{-1/2}$ where $cov(\mathbf{X}) = \boldsymbol{\Sigma}$
2. Take $\mathbf{W} := \hat{\boldsymbol{\Sigma}}^{-1/2}$ and $\mathbf{Z} := \mathbf{X}\mathbf{W}$
3. Apply preferred feature selection procedure with whitened design matrix $Z$ and response $\boldsymbol{Y}$
4. Compute OLS estimates (or other preferred estimators) on corresponding selected subset in $\mathbf{X}$

# 2 Correlation Structures

As discussed in the main text, we consider two different correlation regimes in the simulation study, an autoregressive and block structure. The two structures, with appropriately high parameter values, can both represent strong collinearity. However, they are very different and proxy different types of real data settings. This can be appreciated in terms of eigenvalue decay. For example, considering $\alpha = 0.9$ and $(\rho, \omega) = (0.5, 0.4)$ in simulations with $p = 100$ and $k_0 = 10$, Figure 1 shows the percentage of variance explained by the first 10 eigenvalues. The autoregressive structure has a much steadier decay compared to the block structure – which has a very dominant first component followed by a sharp drop. The autoregressive structure though also has, in a way, a lower intrinsic dimensionality; its first 10 eigenvalues capture around 98% of the overall variability, while the first 10 eigenvalues of the block structure only reach 37%. In our experiments we investigated

both structures with varying parameter values. Due to space limitations, the main text refers only to the autoregressive structure (the most commonly explored in recent articles, see Bertsimas et al. (2016), Hastie et al. (2017), Bertsimas & Van Parys (2017)) – but we report the remaining results in Sections 3 and 4 of this document.

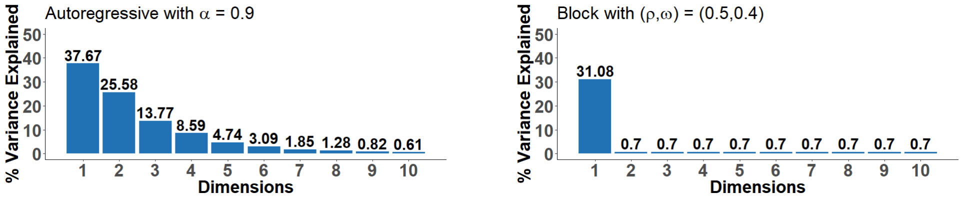


**Figure 1:** Scree plots illustrating eigenvalue decay in autoregressive and block correlation structures.

# 3 Whitening Comparisons

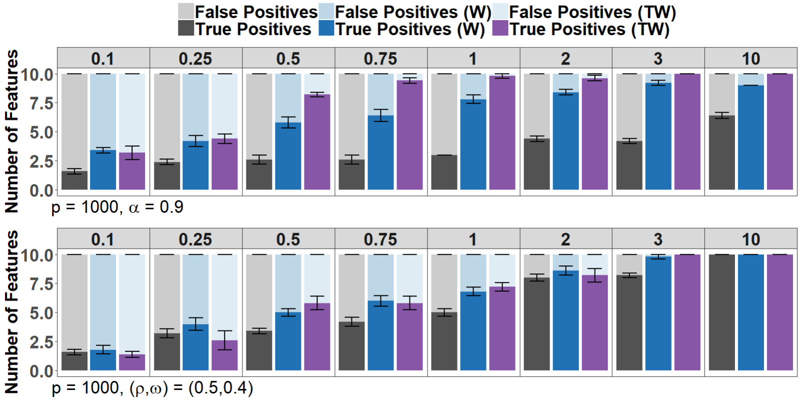


**Figure 2:** Breakdown in average numbers of true and false positives (with error bars at $+/-1SD$) selected solving MIQPs across a range of SNR values (displayed along the top $x$-axis). The data are simulated from scenarios with $p = 1000$, $k_0 = 10$, and highly correlated features with an autoregressive structure (top panel, $\alpha = 0.9$) and a block structure (bottom panel, $(\rho, \omega) = (0.5, 0.4)$). Results are without whitening (gray), with using the MLE of the covariance (blue), and with using the true covariance (purple).

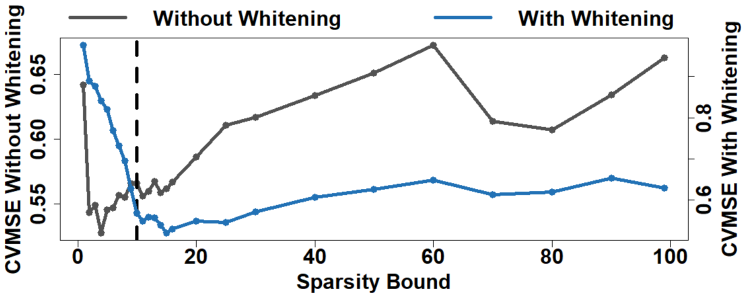


**Figure 3:** Cross-validation Mean Squared Errors with (blue) and without (gray) whitening at SNR=1 for the autoregressive structure. The dashed vertical line marks the true value of the sparsity bound. An additional benefit of ZCA whitening is the effect it has on CVMSE curves. Curves evaluated over $k$ from 1 to $p = 100$ before and after whitening. Using $\mathbf{X}$, noise makes it difficult to identify an appropriate sparsity bound; simply selecting the minimum leads to an excessively sparse solution. Using $\mathbf{Z}$ produces a more distinct elbow behavior, so we can get reasonably close to the true $k_0 = 10$.

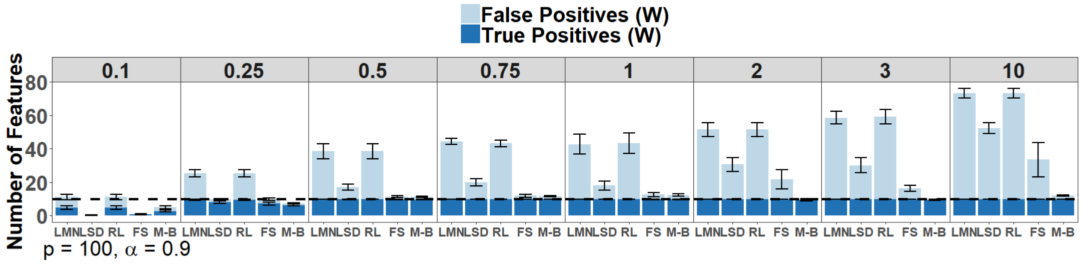


**(a)** Average number of true and false positives over simulation replicates. Bars: $\pm 1SD$, dashed line: $k_o = 10$.

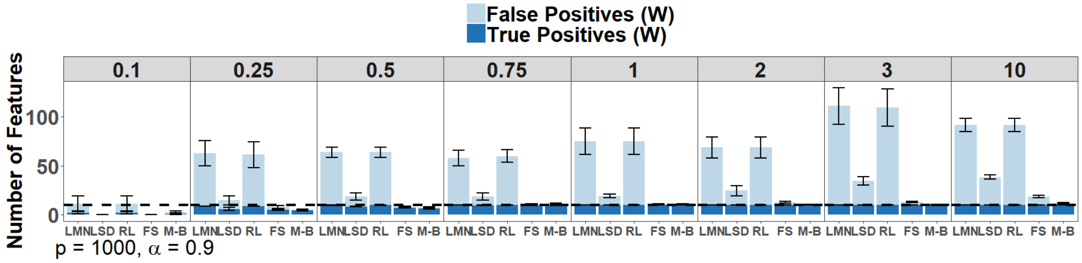


**(b)** Average number of true and false positives over simulation replicates. Bars: $\pm 1SD$, dashed line: $k_o = 10$.

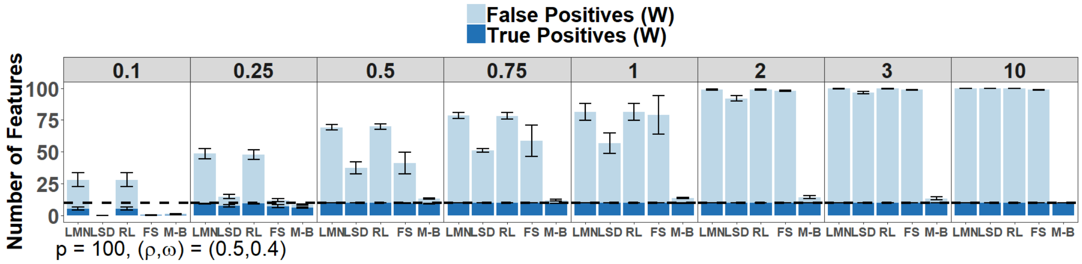


**(c)** Average number of true and false positives over simulation replicates. Bars: $\pm 1SD$, dashed line: $k_o = 10$.

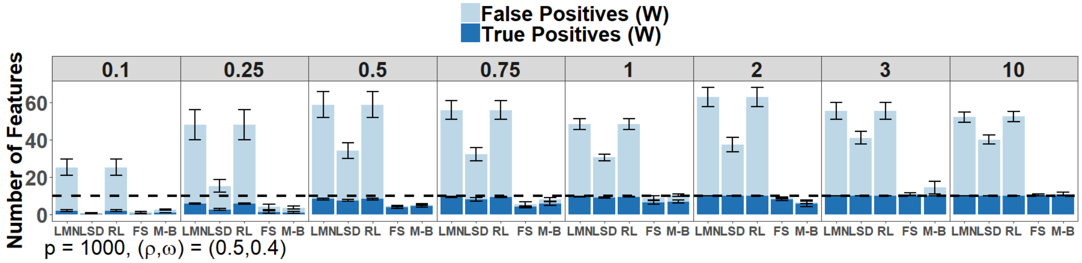


**(d)** Average number of true and false positives over simulation replicates. Bars: $\pm 1SD$, dashed line: $k_o = 10$.

**Figure 4:** Scenarios with $p = 100$, $p = 1000$, $k_o = 10$, various SNR values, autoregressive correlation structure with $\alpha = 0.9$, and block correlation structure with $(\rho, \omega) = (0.5, 0.4)$. Data are whitened in all cases.

# 4 Full Results for Statistical Quality

## 4.1 Scenarios with $p = 100$ and constant $\beta$ coefficients

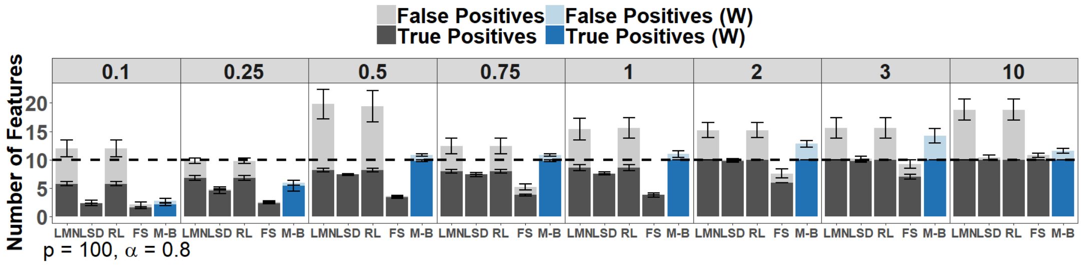


**(a)** Average number of true and false positives over simulation replicates. Bars: $\pm 1SD$, dashed line: $k_o = 10$.

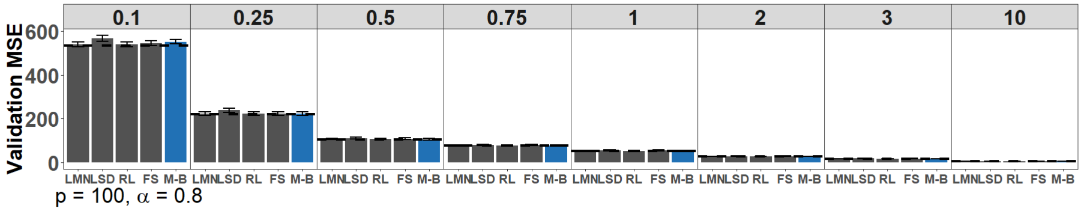


**(b)** Average validation Mean Squared Error over simulation replicates (error bars at $+/-1SD$). Dashed line: error with an OLS fit on the relevant features.

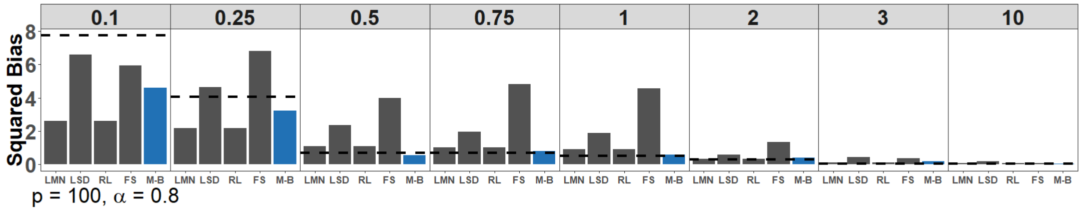


**(c)** Squared bias of $\hat{\beta}$ over simulation replicates. Dashed line: squared bias with an OLS fit on relevant features.

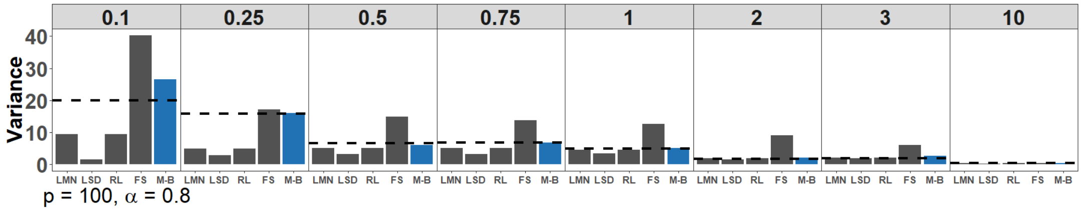


**(d)** Variance of $\hat{\beta}$ over simulation replicates. Dashed line: variance with an OLS fit on relevant features.

**Figure 5:** Summary results in scenarios with $p = 100$, $k_0 = 10$, various SNR values, and autoregressive correlation structure with $\alpha = 0.8$. Blue: data whitened using the MLE of the covariance (MIP BF and MIP BVR). Gray: original data.

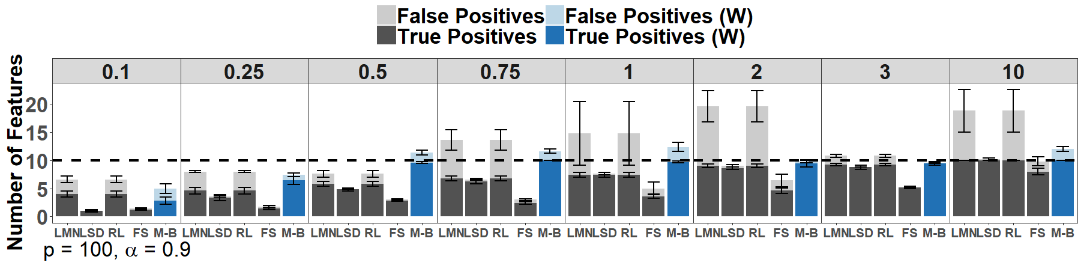


**(a)** Average number of true and false positives over simulation replicates. Bars: $\pm 1SD$, dashed line: $k_o = 10$.

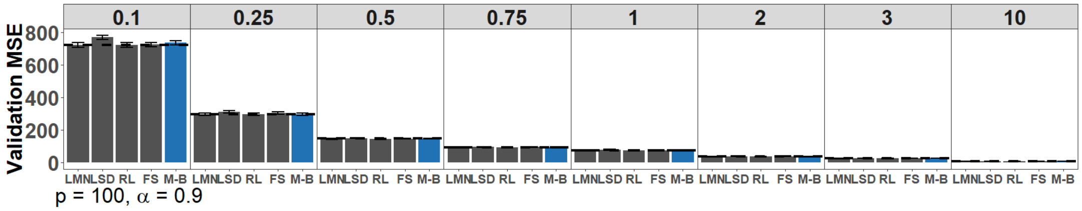


**(b)** Average validation Mean Squared Error over simulation replicates (error bars at $+/-1SD$). Dashed line: error with an OLS fit on the relevant features.

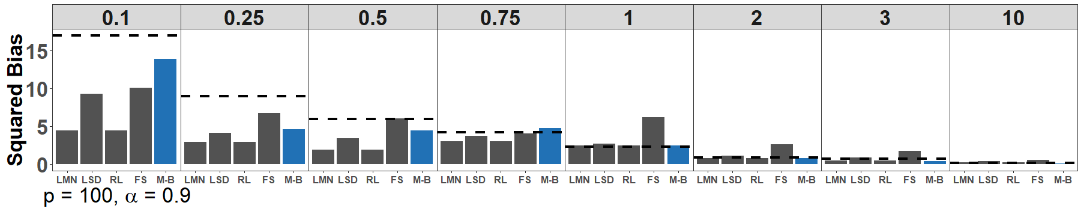


**(c)** Squared bias of $\hat{\beta}$ over simulation replicates. Dashed line: squared bias with an OLS fit on relevant features.

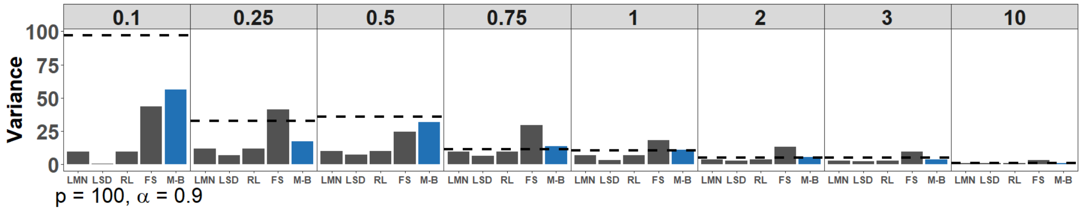


**(d)** Variance of $\hat{\beta}$ over simulation replicates. Dashed line: variance with an OLS fit on relevant features.

**Figure 6:** Summary results in scenarios with $p = 100$, $k_0 = 10$, various SNR values, and autoregressive correlation structure with $\alpha = 0.9$. Blue: data whitened using the MLE of the covariance (MIP BF and MIP BVR). Gray: original data. For SNR $\leq 0.75$ we performed 10 trials (rather than 5) to better account for the high variability from noise. All other scenarios have 5 due to the computational burden of MIP methods.

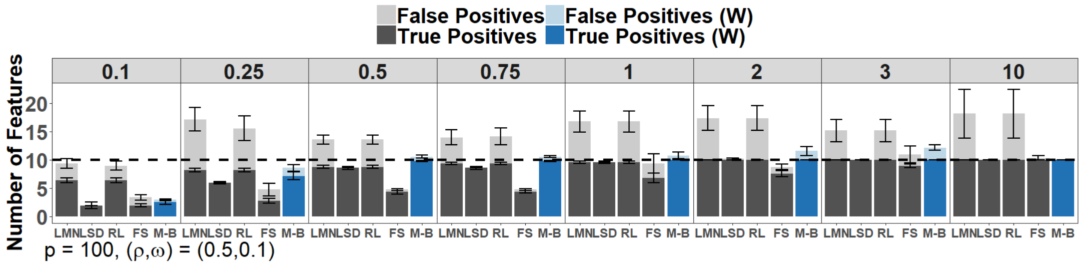


**(a)** Average number of true and false positives over simulation replicates. Bars: $\pm 1SD$, dashed line: $k_o = 10$.

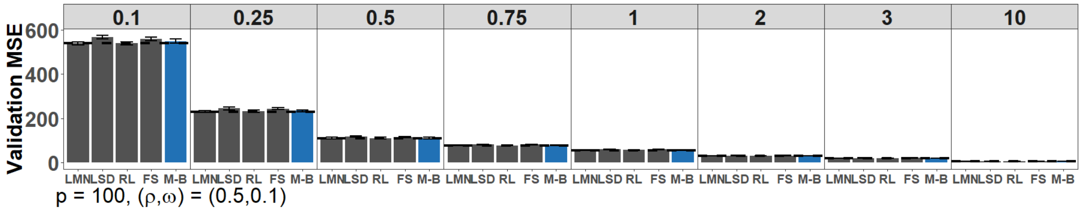


**(b)** Average validation Mean Squared Error over simulation replicates (error bars at $+/-1SD$). Dashed line: error with an OLS fit on the relevant features.

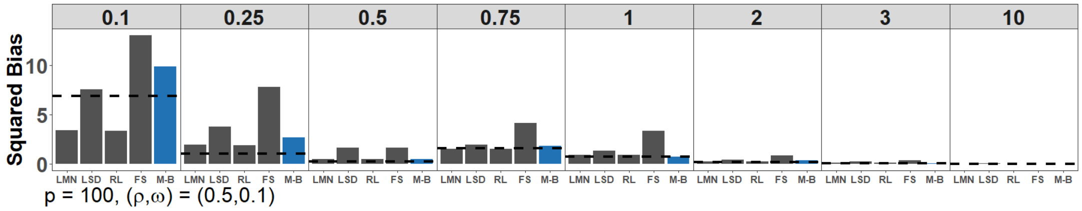


**(c)** Squared bias of $\hat{\beta}$ over simulation replicates. Dashed line: squared bias with an OLS fit on relevant features.

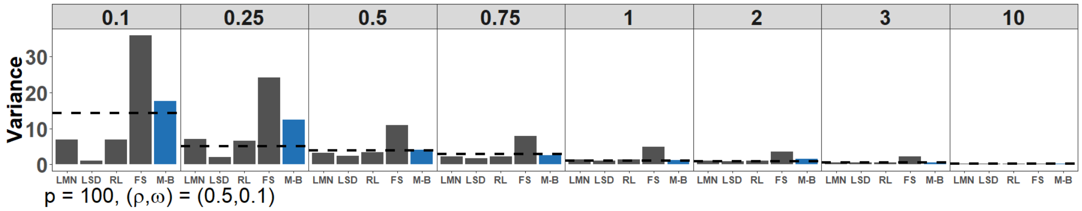


**(d)** Variance of $\hat{\beta}$ over simulation replicates. Dashed line: variance with an OLS fit on relevant features.

**Figure 7:** Summary results in scenarios with $p = 100$, $k_0 = 10$, various SNR values, and block correlation structure with $(\rho, \omega) = (0.5, 0.1)$. Blue: data whitened using the MLE of the covariance (MIP BF and MIP BVR). Gray: original data.

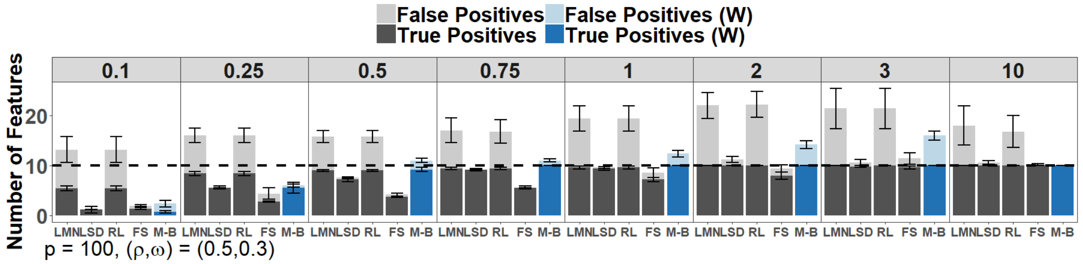


**(a)** Average number of true and false positives over simulation replicates. Bars: $\pm 1SD$, dashed line: $k_o = 10$.

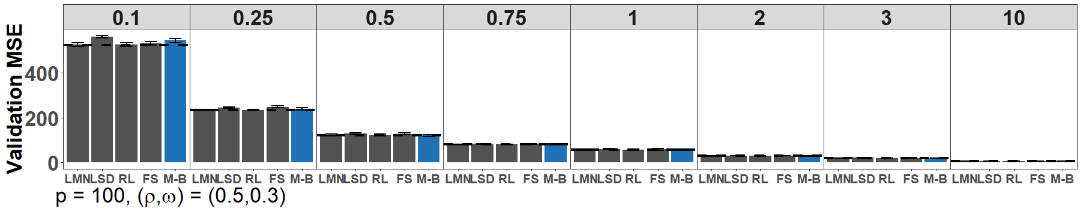


**(b)** Average validation Mean Squared Error over simulation replicates (error bars at $+/-1SD$). Dashed line: error with an OLS fit on the relevant features.

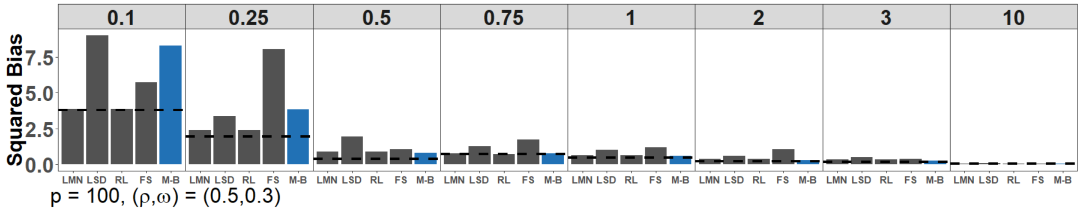


**(c)** Squared bias of $\hat{\beta}$ over simulation replicates. Dashed line: squared bias with an OLS fit on relevant features.

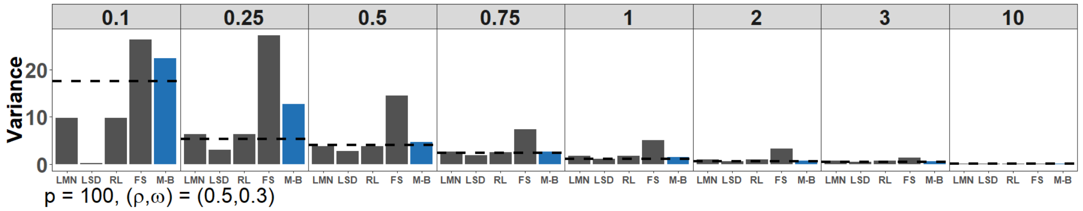


**(d)** Variance of $\hat{\beta}$ over simulation replicates. Dashed line: variance with an OLS fit on relevant features.

**Figure 8:** Summary results in scenarios with $p = 100$, $k_0 = 10$, various SNR values, and block correlation structure with $(\rho, \omega) = (0.5, 0.3)$. Blue: data whitened using the MLE of the covariance (MIP BF and MIP BVR). Gray: original data.

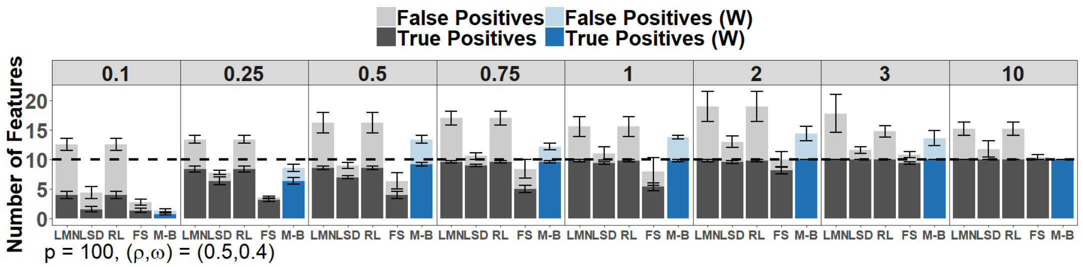


**(a)** Average number of true and false positives over simulation replicates. Bars: $\pm 1SD$, dashed line: $k_o = 10$.

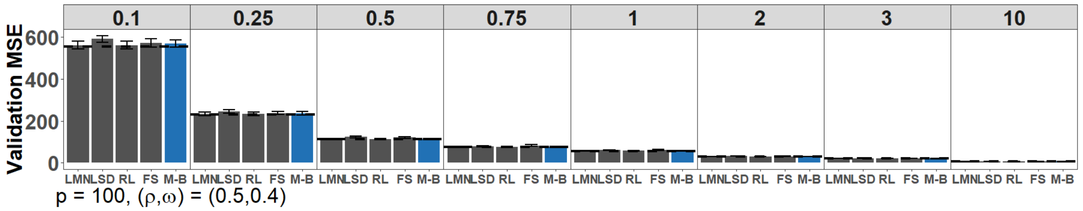


**(b)** Average validation Mean Squared Error over simulation replicates (error bars at $+/-1SD$). Dashed line: error with an OLS fit on the relevant features.

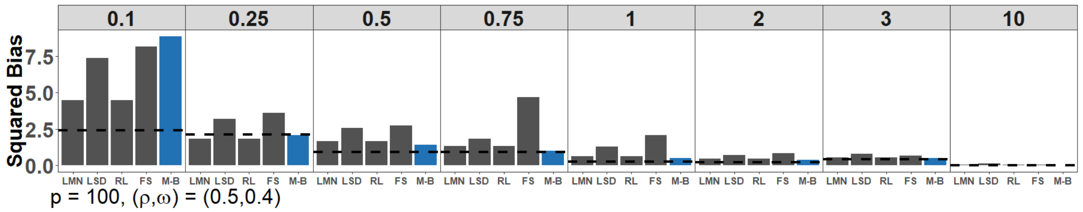


**(c)** Squared bias of $\hat{\beta}$ over simulation replicates. Dashed line: squared bias with an OLS fit on relevant features.

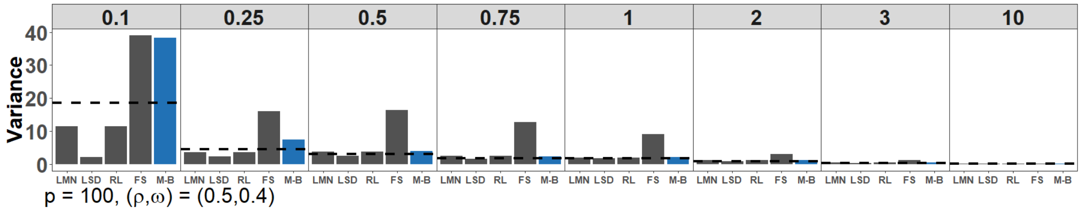


**(d)** Variance of $\hat{\beta}$ over simulation replicates. Dashed line: variance with an OLS fit on relevant features.

**Figure 9:** Summary results in scenarios with $p = 100$, $k_0 = 10$, various SNR values, and block correlation structure with $(\rho, \omega) = (0.5, 0.4)$. Blue: data whitened using the MLE of the covariance (MIP BF and MIP BVR). Gray: original data.

## 4.2 Scenarios with $p = 100$ and varying $\beta$ coefficients

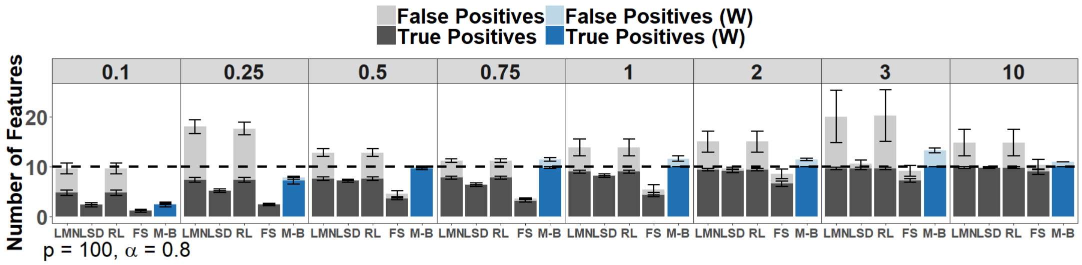


**(a)** Average number of true and false positives over simulation replicates. Bars: $\pm 1SD$, dashed line: $k_o = 10$.

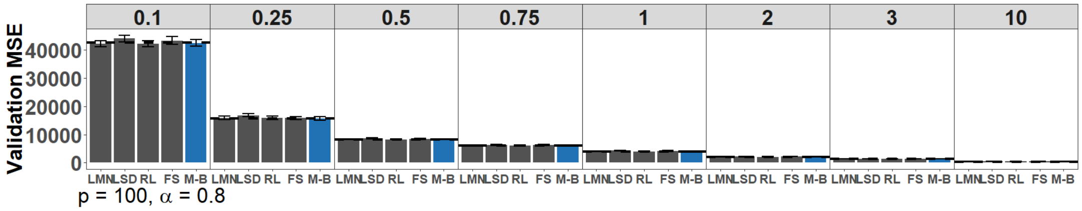


**(b)** Average validation Mean Squared Error over simulation replicates (error bars at $+/-1SD$). Dashed line: error with an OLS fit on the relevant features.

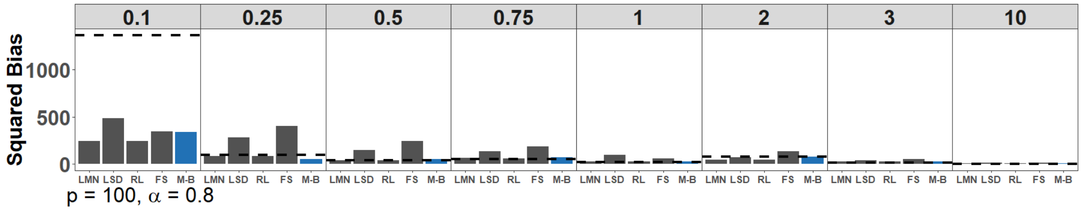


**(c)** Squared bias of $\hat{\beta}$ over simulation replicates. Dashed line: squared bias with an OLS fit on relevant features.

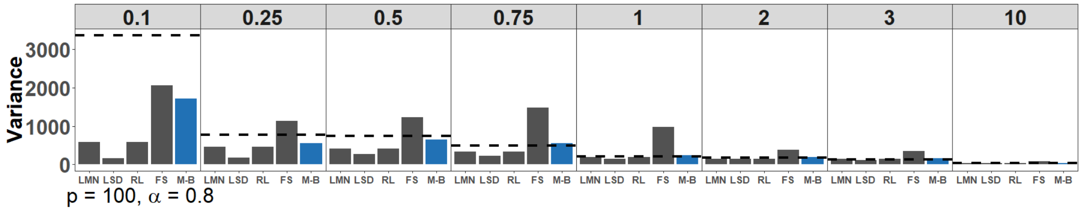


**(d)** Variance of $\hat{\beta}$ over simulation replicates. Dashed line: variance with an OLS fit on relevant features.

**Figure 10:** Summary results in scenarios with $p = 100$, $k_0 = 10$, various SNR values, and autoregressive correlation structure with $\alpha = 0.8$. Blue: data whitened using the MLE of the covariance (MIP BF and MIP BVR). Gray: original data.

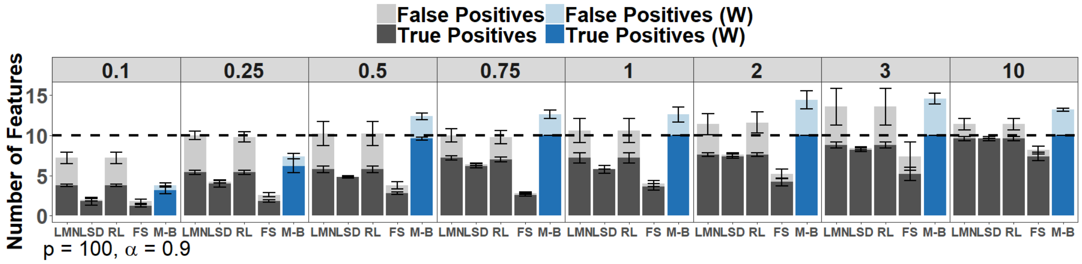


**(a)** Average number of true and false positives over simulation replicates. Bars: $\pm 1SD$, dashed line: $k_o = 10$.

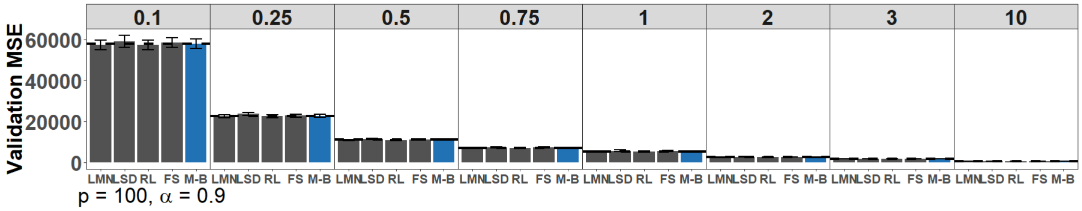


**(b)** Average validation Mean Squared Error over simulation replicates (error bars at $+/-1SD$). Dashed line: error with an OLS fit on the relevant features.

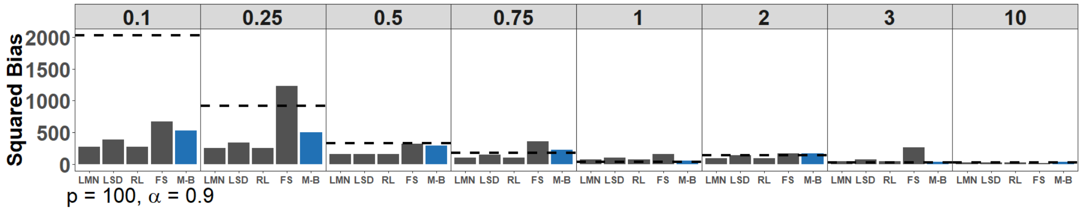


**(c)** Squared bias of $\hat{\beta}$ over simulation replicates. Dashed line: squared bias with an OLS fit on relevant features.

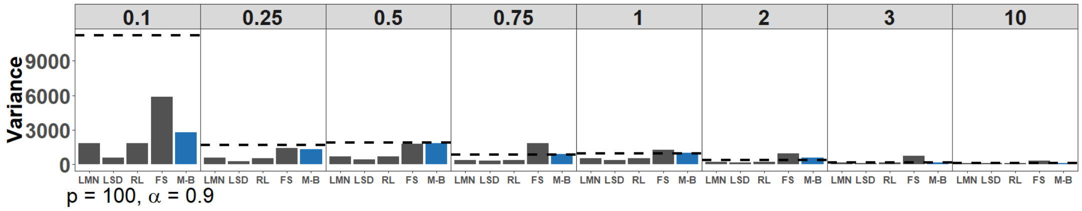


**(d)** Variance of $\hat{\beta}$ over simulation replicates. Dashed line: variance with an OLS fit on relevant features.

**Figure 11:** Summary results in scenarios with $p = 100$, $k_0 = 10$, various SNR values, and autoregressive correlation structure with $\alpha = 0.9$. Blue: data whitened using the MLE of the covariance (MIP BF and MIP BVR). Gray: original data.

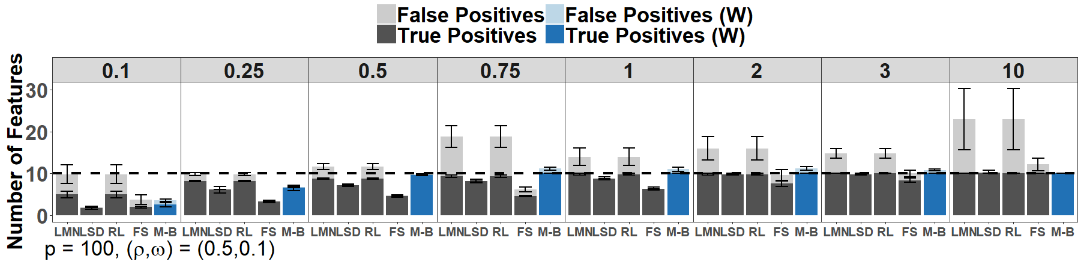


**(a)** Average number of true and false positives over simulation replicates. Bars: $\pm 1SD$, dashed line: $k_o = 10$.

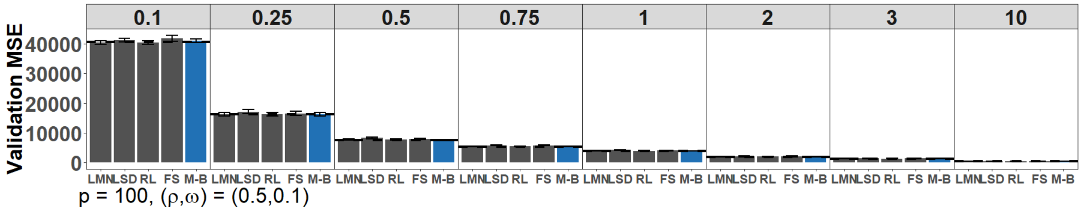


**(b)** Average validation Mean Squared Error over simulation replicates (error bars at $+/-1SD$). Dashed line: error with an OLS fit on the relevant features.

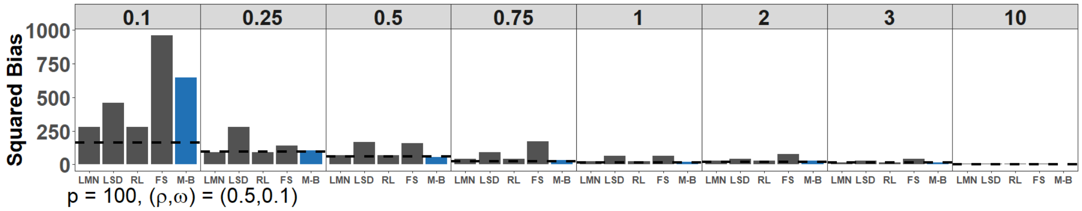


**(c)** Squared bias of $\hat{\beta}$ over simulation replicates. Dashed line: squared bias with an OLS fit on relevant features.

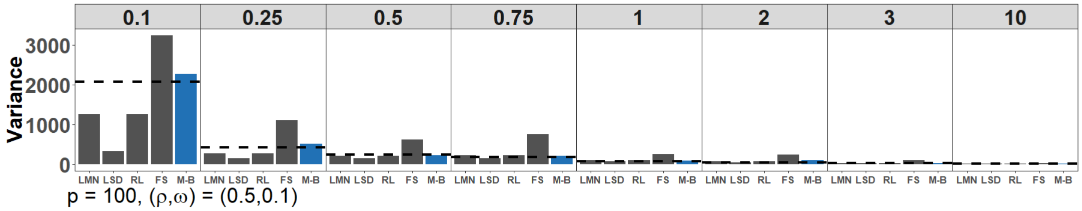


**(d)** Variance of $\hat{\beta}$ over simulation replicates. Dashed line: variance with an OLS fit on relevant features.

**Figure 12:** Summary results in scenarios with $p = 100$, $k_0 = 10$, various SNR values, and block correlation structure with $(\rho, \omega) = (0.5, 0.1)$. Blue: data whitened using the MLE of the covariance (MIP BF and MIP BVR). Gray: original data.

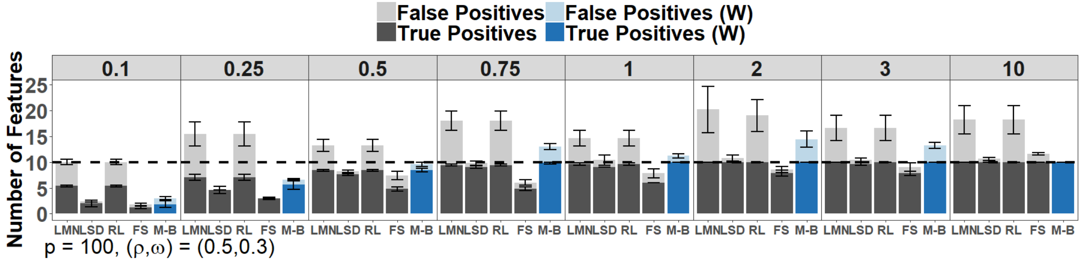


**(a)** Average number of true and false positives over simulation replicates. Bars: $\pm 1SD$, dashed line: $k_o = 10$.

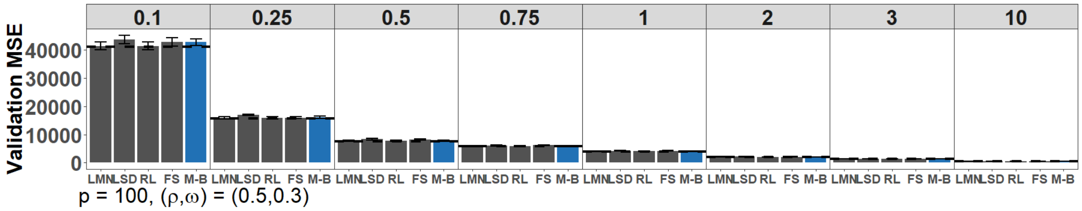


**(b)** Average validation Mean Squared Error over simulation replicates (error bars at $+/-1SD$). Dashed line: error with an OLS fit on the relevant features.

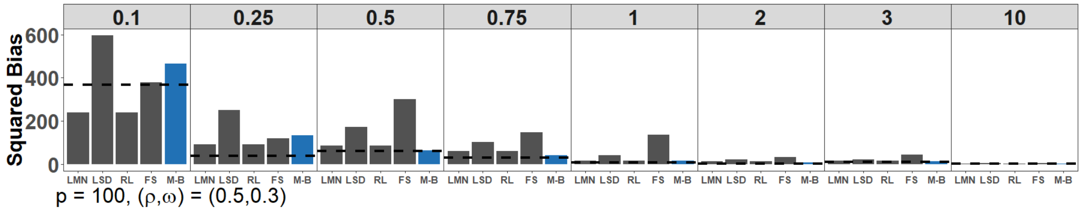


**(c)** Squared bias of $\hat{\beta}$ over simulation replicates. Dashed line: squared bias with an OLS fit on relevant features.

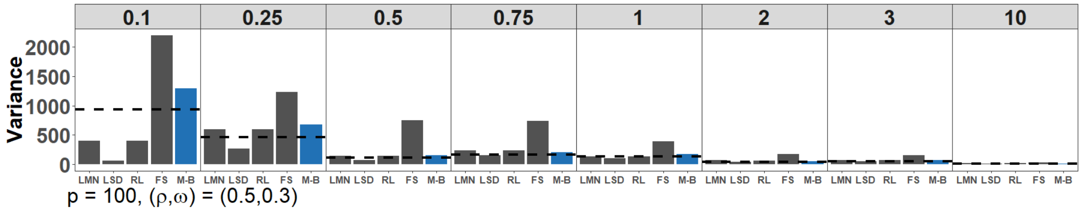


**(d)** Variance of $\hat{\beta}$ over simulation replicates. Dashed line: variance with an OLS fit on relevant features.

**Figure 13:** Summary results in scenarios with $p = 100$, $k_0 = 10$, various SNR values, and block correlation structure with $(\rho, \omega) = (0.5, 0.3)$. Blue: data whitened using the MLE of the covariance (MIP BF and MIP BVR). Gray: original data.

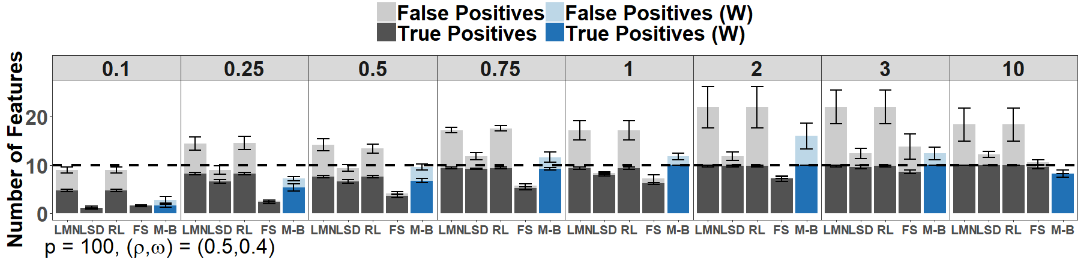


**(a)** Average number of true and false positives over simulation replicates. Bars: $\pm 1SD$, dashed line: $k_o = 10$.

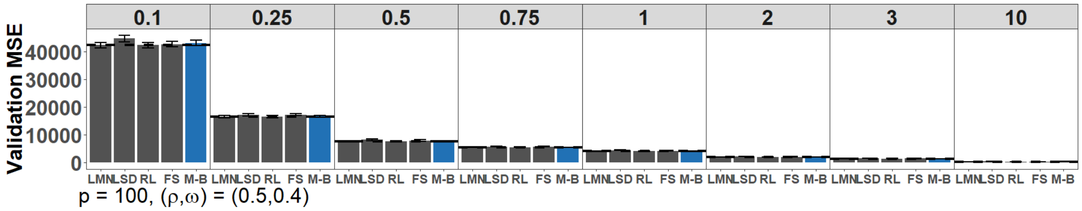


**(b)** Average validation Mean Squared Error over simulation replicates (error bars at $+/-1SD$). Dashed line: error with an OLS fit on the relevant features.

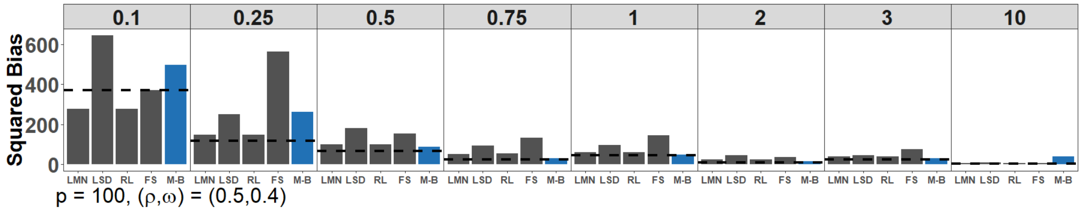


**(c)** Squared bias of $\hat{\beta}$ over simulation replicates. Dashed line: squared bias with an OLS fit on relevant features.

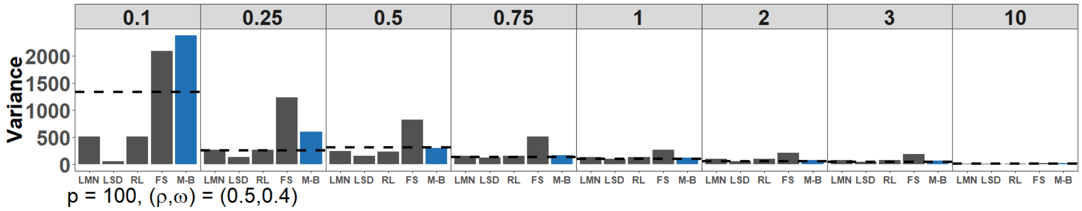


**(d)** Variance of $\hat{\beta}$ over simulation replicates. Dashed line: variance with an OLS fit on relevant features.

**Figure 14:** Summary results in scenarios with $p = 100$, $k_0 = 10$, various SNR values, and block correlation structure with $(\rho, \omega) = (0.5, 0.4)$. Blue: data whitened using the MLE of the covariance (MIP BF and MIP BVR). Gray: original data.

## 4.3 Scenarios with $p = 1000$ and constant $\beta$ coefficients

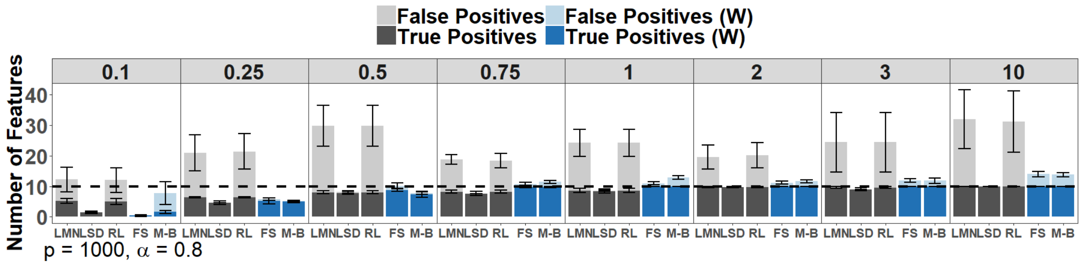


**(a)** Average number of true and false positives over simulation replicates. Bars: $\pm 1SD$, dashed line: $k_o = 10$.

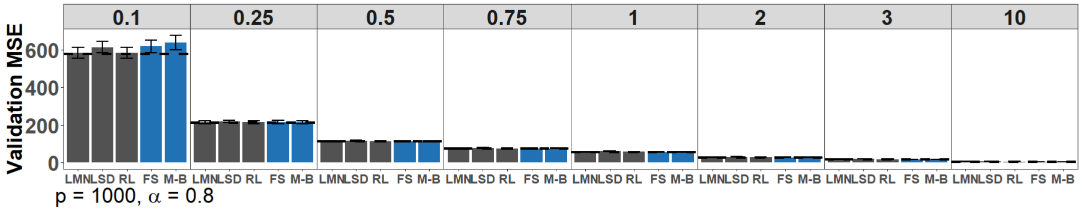


**(b)** Average validation Mean Squared Error over simulation replicates (error bars at $+/-1SD$). Dashed line: error with an OLS fit on the relevant features.

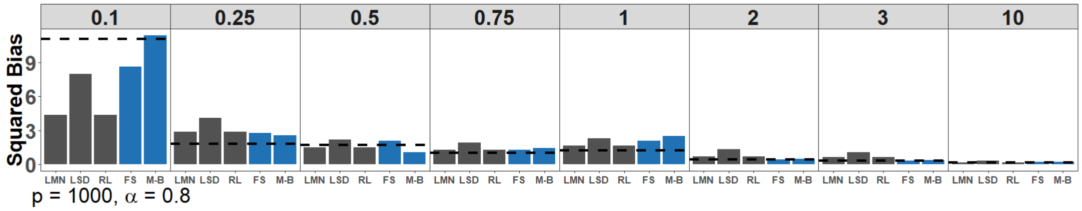


**(c)** Squared bias of $\hat{\beta}$ over simulation replicates. Dashed line: squared bias with an OLS fit on relevant features.

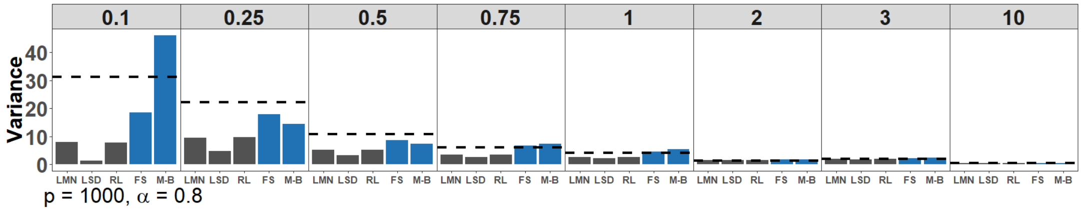


**(d)** Variance of $\hat{\beta}$ over simulation replicates. Dashed line: variance with an OLS fit on relevant features.

**Figure 15:** Summary results in scenarios with $p = 1000$, $k_0 = 10$, various SNR values, and autoregressive correlation structure with $\alpha = 0.8$. Purple: data whitened using the true covariance (MIP BF, MIP BVR, and FS). Gray: original data.

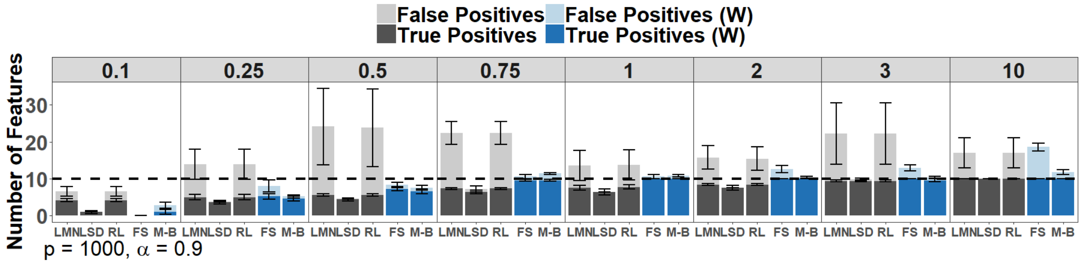


**(a)** Average number of true and false positives over simulation replicates. Bars: $\pm 1SD$, dashed line: $k_o = 10$.

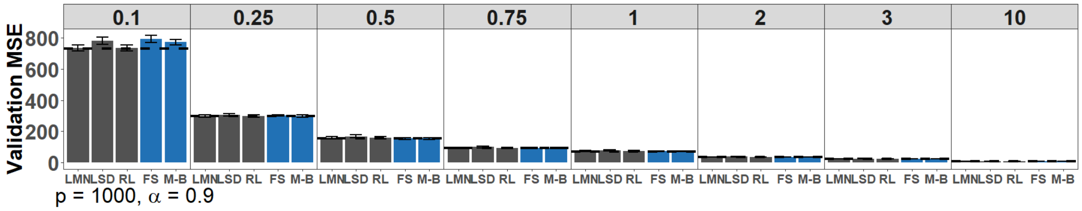


**(b)** Average validation Mean Squared Error over simulation replicates (error bars at $+/-1SD$). Dashed line: error with an OLS fit on the relevant features.

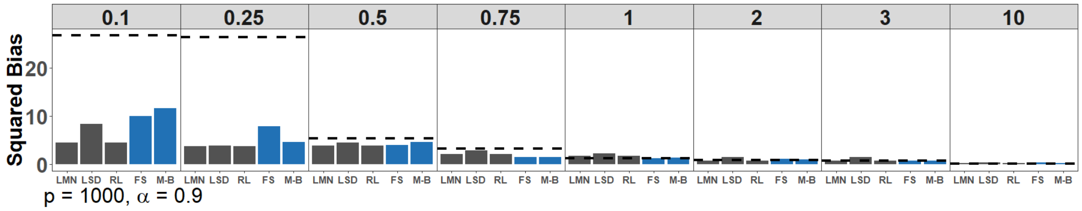


**(c)** Squared bias of $\hat{\beta}$ over simulation replicates. Dashed line: squared bias with an OLS fit on relevant features.

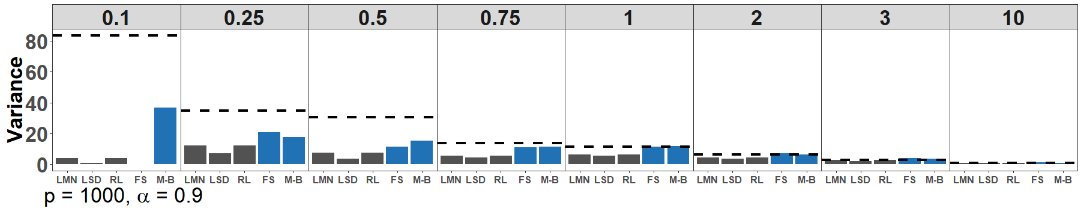


**(d)** Variance of $\hat{\beta}$ over simulation replicates. Dashed line: variance with an OLS fit on relevant features.

**Figure 16:** Summary results in scenarios with $p = 1000$, $k_0 = 10$, various SNR values, and autoregressive correlation structure with $\alpha = 0.9$. Purple: data whitened using the true covariance (MIP BF, MIP BVR, and FS). Gray: original data.

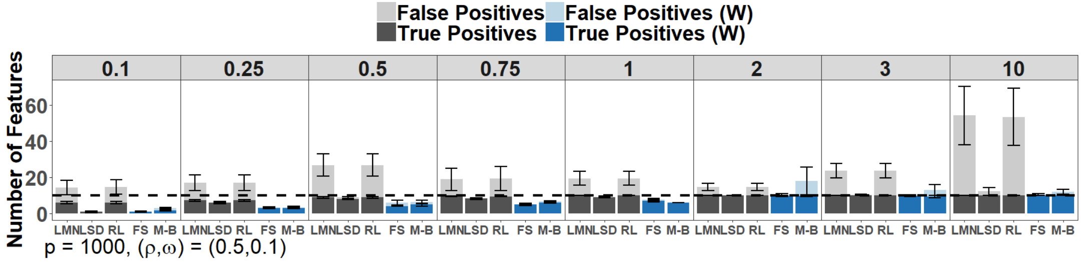


**(a)** Average number of true and false positives over simulation replicates. Bars: $\pm 1SD$, dashed line: $k_o = 10$.

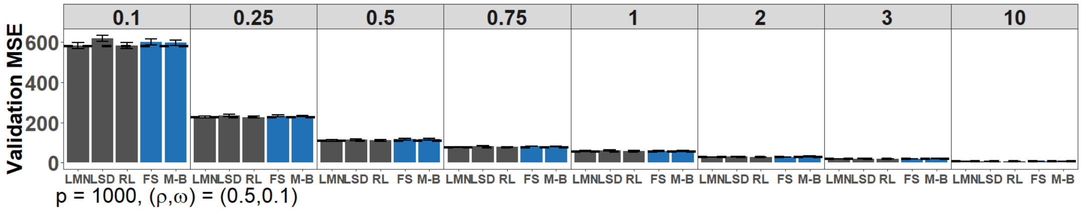


**(b)** Average validation Mean Squared Error over simulation replicates (error bars at $+/-1SD$). Dashed line: error with an OLS fit on the relevant features.

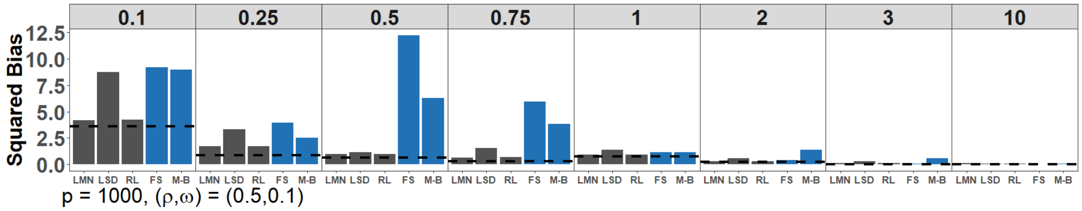


**(c)** Squared bias of $\hat{\beta}$ over simulation replicates. Dashed line: squared bias with an OLS fit on relevant features.

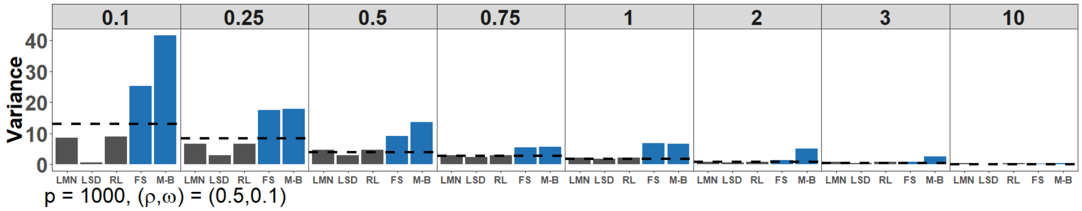


**(d)** Variance of $\hat{\beta}$ over simulation replicates. Dashed line: variance with an OLS fit on relevant features.

**Figure 17:** Summary results in scenarios with $p = 1000$, $k_0 = 10$, various SNR values, and block correlation structure with $(\rho, \omega) = (0.5, 0.1)$. Purple: data whitened using the true covariance (MIP BF, MIP BVR, and FS). Gray: original data.

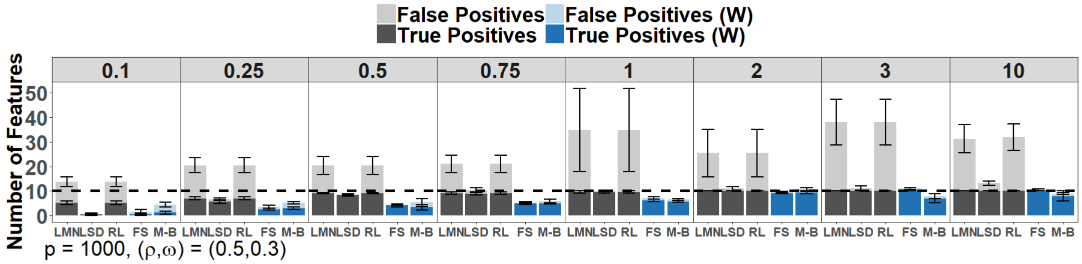


**(a)** Average number of true and false positives over simulation replicates. Bars: $\pm 1SD$, dashed line: $k_o = 10$.

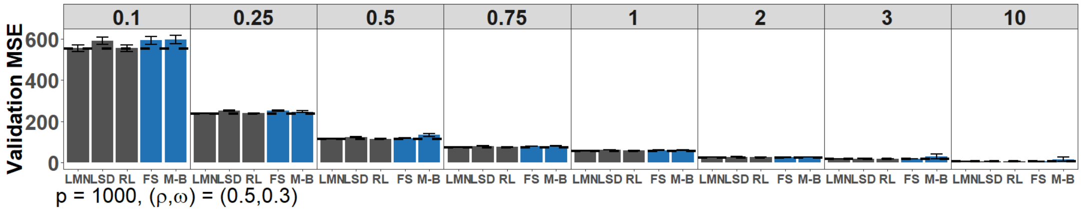


**(b)** Average validation Mean Squared Error over simulation replicates (error bars at $+/-1SD$). Dashed line: error with an OLS fit on the relevant features.

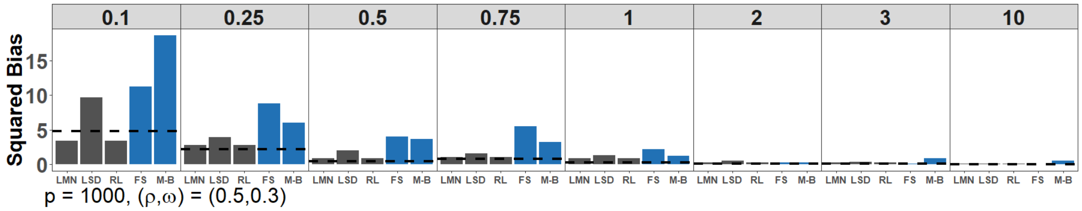


**(c)** Squared bias of $\hat{\beta}$ over simulation replicates. Dashed line: squared bias with an OLS fit on relevant features.

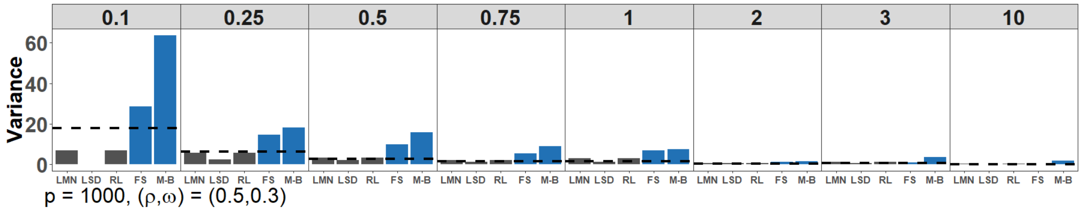


**(d)** Variance of $\hat{\beta}$ over simulation replicates. Dashed line: variance with an OLS fit on relevant features.

**Figure 18:** Summary results in scenarios with $p = 1000$, $k_0 = 10$, various SNR values, and block correlation structure with $(\rho, \omega) = (0.5, 0.3)$. Purple: data whitened using the true covariance (MIP BF, MIP BVR, and FS). Gray: original data.

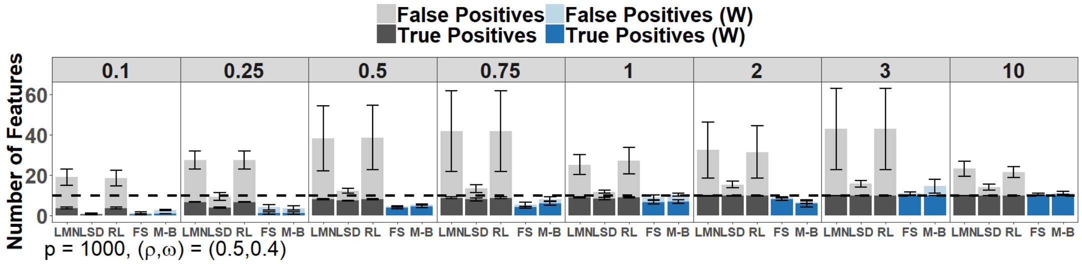


**(a)** Average number of true and false positives over simulation replicates. Bars: $\pm 1SD$, dashed line: $k_o = 10$.

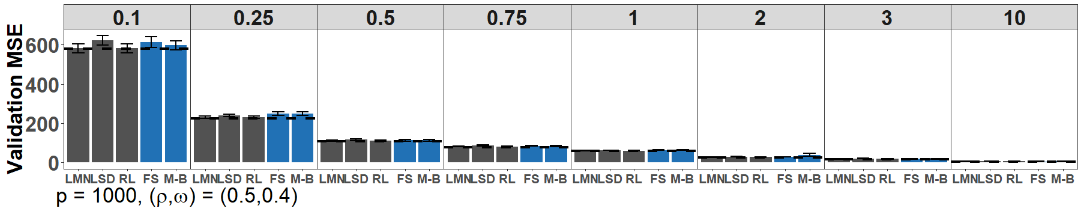


**(b)** Average validation Mean Squared Error over simulation replicates (error bars at $+/-1SD$). Dashed line: error with an OLS fit on the relevant features.

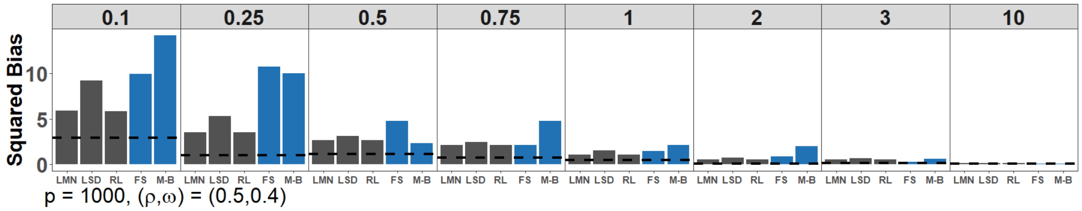


**(c)** Squared bias of $\hat{\beta}$ over simulation replicates. Dashed line: squared bias with an OLS fit on relevant features.

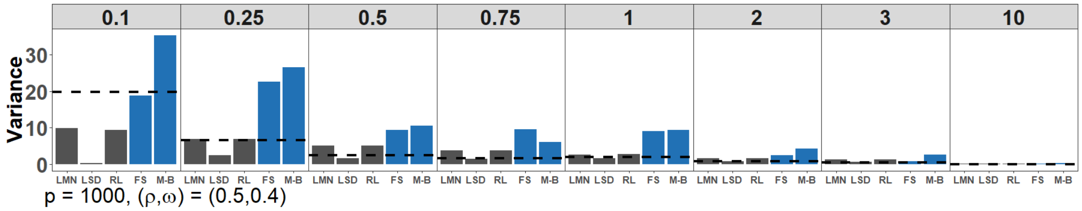


**(d)** Variance of $\hat{\beta}$ over simulation replicates. Dashed line: variance with an OLS fit on relevant features.

**Figure 19:** Summary results in scenarios with $p = 1000$, $k_0 = 10$, various SNR values, and block correlation structure with $(\rho, \omega) = (0.5, 0.4)$. Purple: data whitened using the true covariance (MIP BF, MIP BVR, and FS). Gray: original data.

## 4.4 Scenarios with $p = 1000$ and varying $\beta$ coefficients

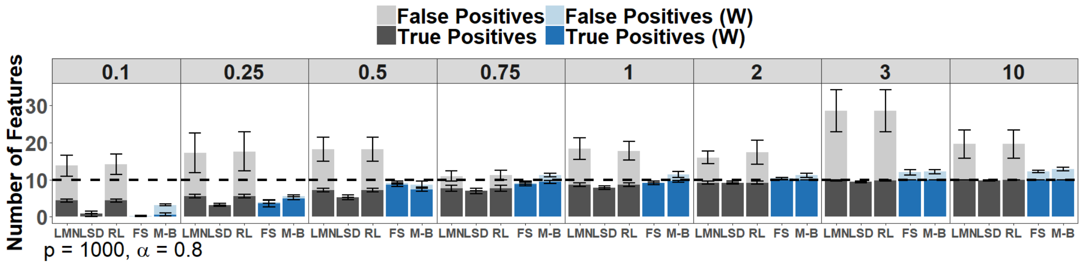


**(a)** Average number of true and false positives over simulation replicates. Bars: $\pm 1SD$, dashed line: $k_o = 10$.

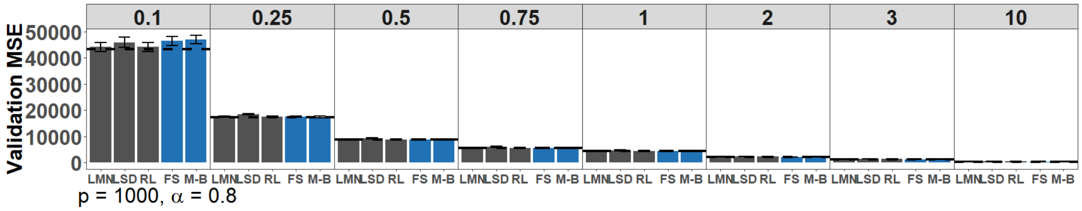


**(b)** Average validation Mean Squared Error over simulation replicates (error bars at $+/-1SD$). Dashed line: error with an OLS fit on the relevant features.

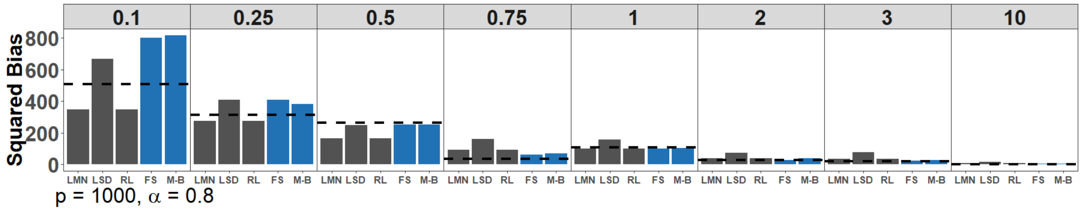


**(c)** Squared bias of $\hat{\beta}$ over simulation replicates. Dashed line: squared bias with an OLS fit on relevant features.

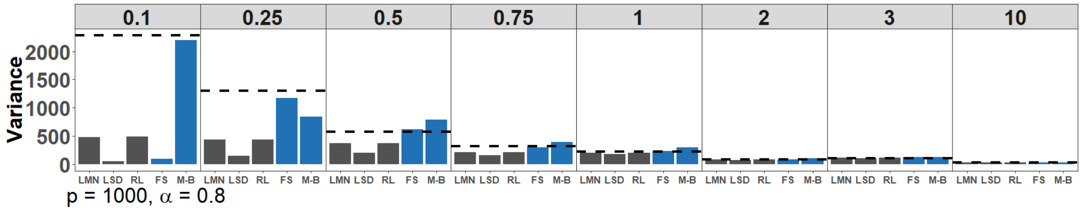


**(d)** Variance of $\hat{\beta}$ over simulation replicates. Dashed line: variance with an OLS fit on relevant features.

**Figure 20:** Summary results in scenarios with $p = 1000$, $k_0 = 10$, various SNR values, and autoregressive correlation structure with $\alpha = 0.8$. Purple: data whitened using the true covariance (MIP BF, MIP BVR, and FS). Gray: original data.

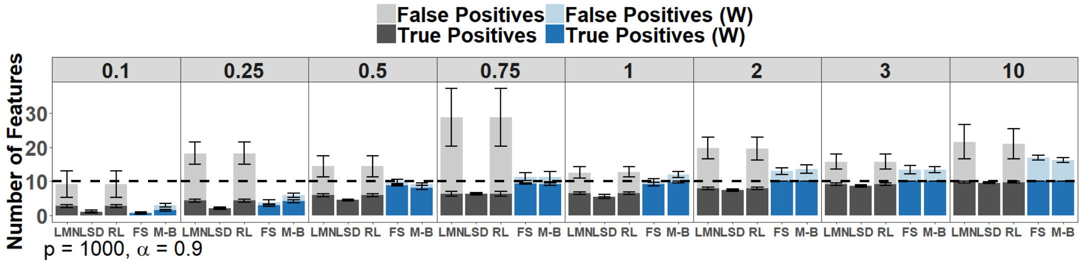


**(a)** Average number of true and false positives over simulation replicates. Bars: $\pm 1SD$, dashed line: $k_o = 10$.

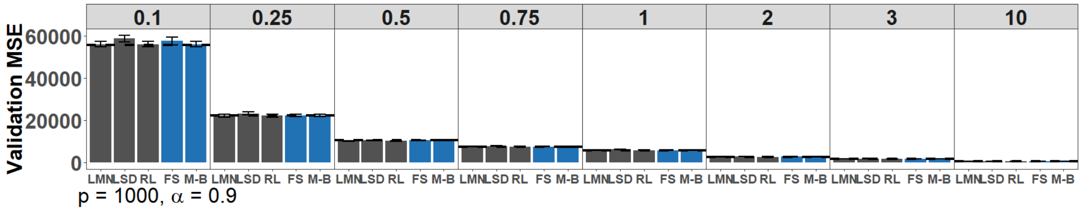


**(b)** Average validation Mean Squared Error over simulation replicates (error bars at $+/-1SD$). Dashed line: error with an OLS fit on the relevant features.

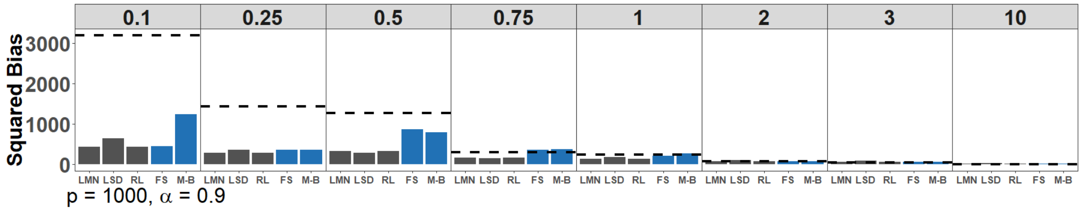


**(c)** Squared bias of $\hat{\beta}$ over simulation replicates. Dashed line: squared bias with an OLS fit on relevant features.

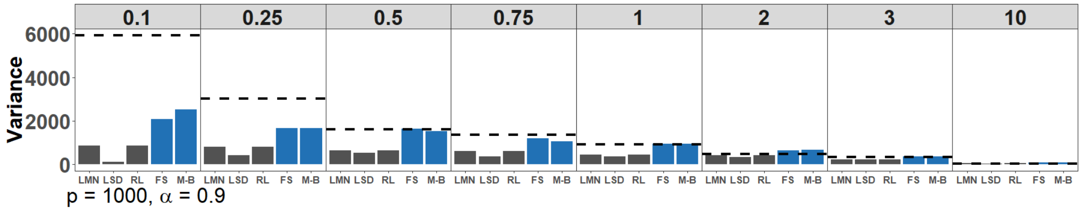


**(d)** Variance of $\hat{\beta}$ over simulation replicates. Dashed line: variance with an OLS fit on relevant features.

**Figure 21:** Summary results in scenarios with $p = 1000$, $k_0 = 10$, various SNR values, and autoregressive correlation structure with $\alpha = 0.9$. Purple: data whitened using the true covariance (MIP BF, MIP BVR, and FS). Gray: original data.

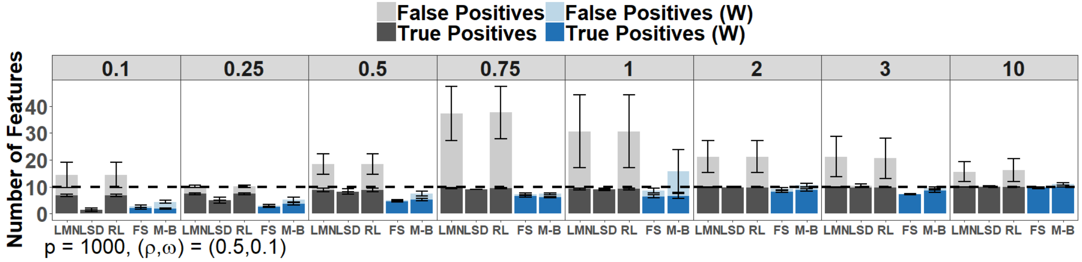


**(a)** Average number of true and false positives over simulation replicates. Bars: $\pm 1SD$, dashed line: $k_o = 10$.

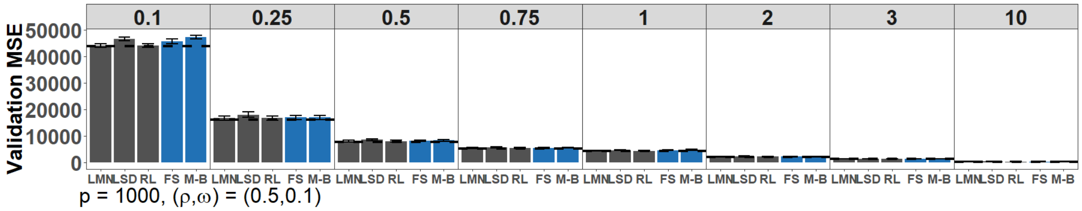


**(b)** Average validation Mean Squared Error over simulation replicates (error bars at $+/-1SD$). Dashed line: error with an OLS fit on the relevant features.

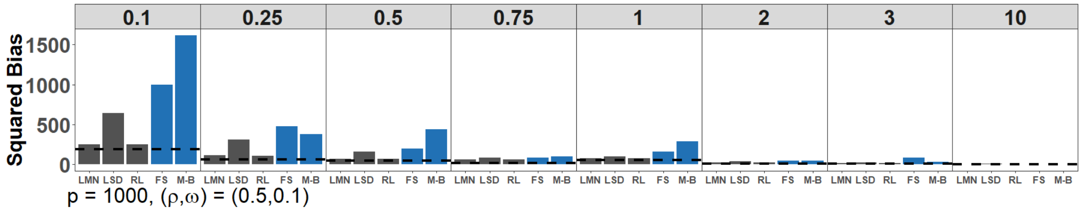


**(c)** Squared bias of $\hat{\beta}$ over simulation replicates. Dashed line: squared bias with an OLS fit on relevant features.

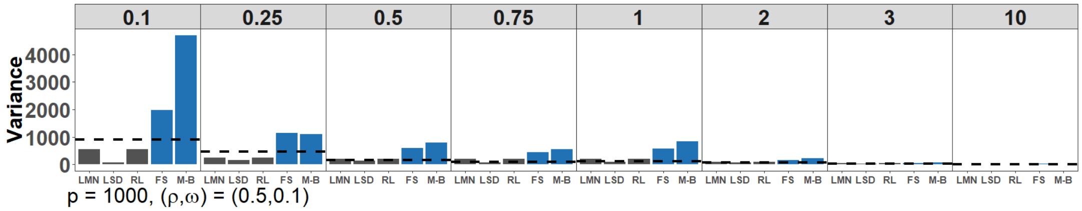


**(d)** Variance of $\hat{\beta}$ over simulation replicates. Dashed line: variance with an OLS fit on relevant features.

**Figure 22:** Summary results in scenarios with $p = 1000$, $k_0 = 10$, various SNR values, and block correlation structure with $(\rho, \omega) = (0.5, 0.1)$. Purple: data whitened using the true covariance (MIP BF, MIP BVR, and FS). Gray: original data.

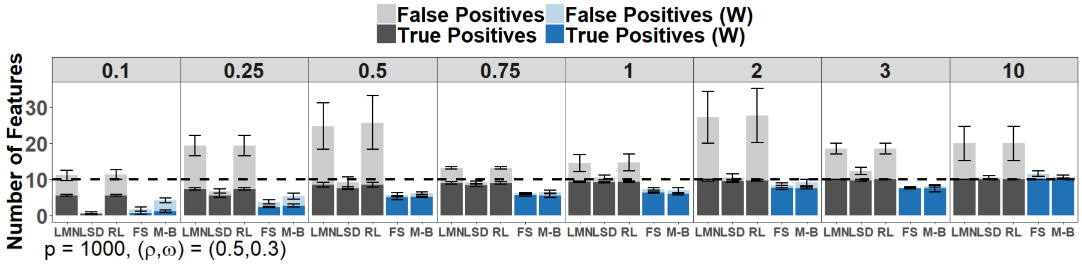


**(a)** Average number of true and false positives over simulation replicates. Bars: $\pm 1SD$, dashed line: $k_o = 10$.

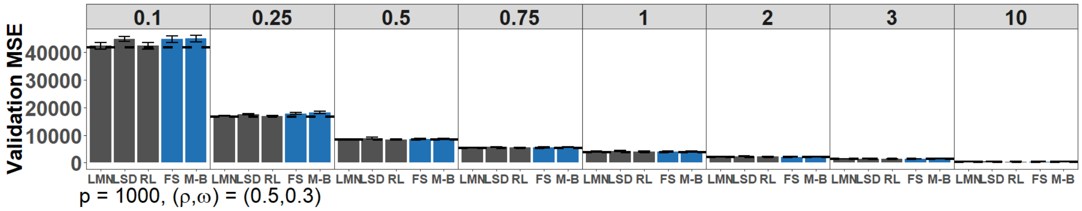


**(b)** Average validation Mean Squared Error over simulation replicates (error bars at $+/-1SD$). Dashed line: error with an OLS fit on the relevant features.

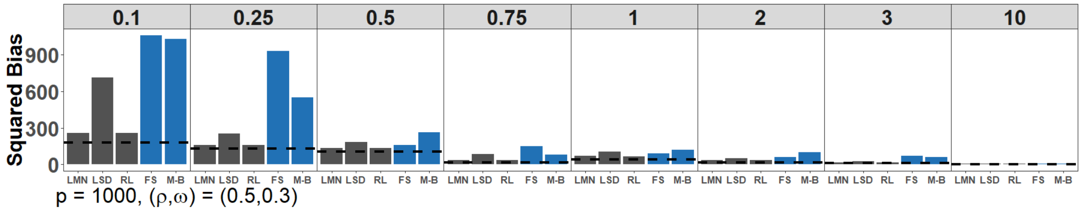


**(c)** Squared bias of $\hat{\beta}$ over simulation replicates. Dashed line: squared bias with an OLS fit on relevant features.

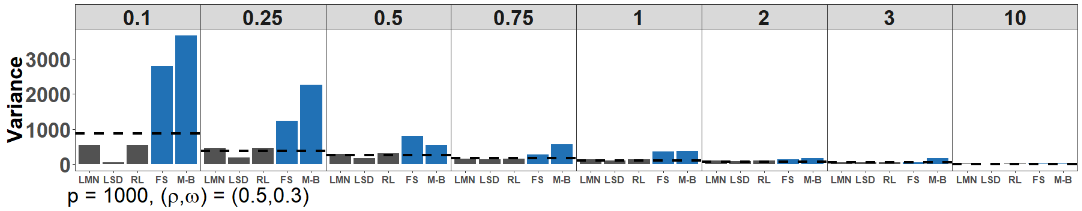


**(d)** Variance of $\hat{\beta}$ over simulation replicates. Dashed line: variance with an OLS fit on relevant features.

**Figure 23:** Summary results in scenarios with $p = 1000$, $k_0 = 10$, various SNR values, and block correlation structure with $(\rho, \omega) = (0.5, 0.3)$. Purple: data whitened using the true covariance (MIP BF, MIP BVR, and FS). Gray: original data.

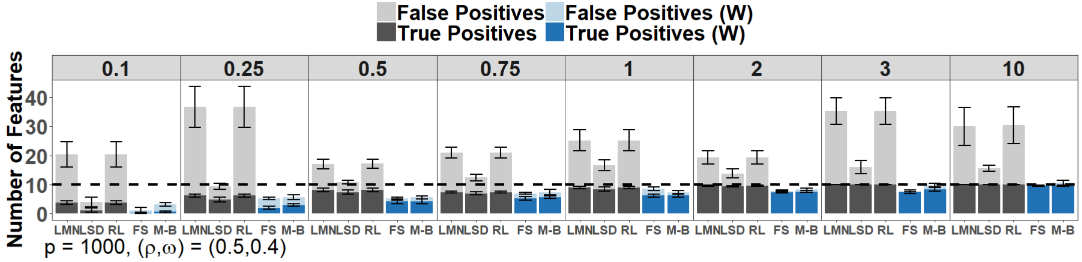


**(a)** Average number of true and false positives over simulation replicates. Bars: $\pm 1SD$, dashed line: $k_o = 10$.

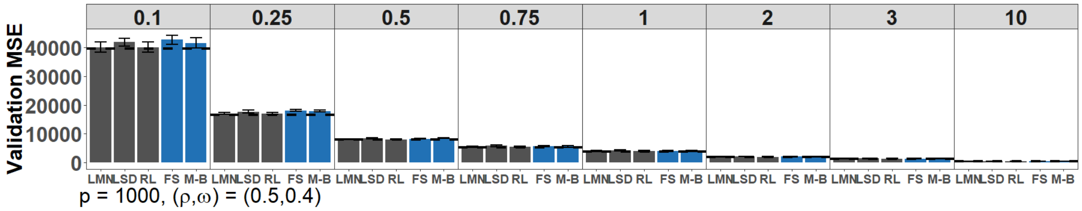


**(b)** Average validation Mean Squared Error over simulation replicates (error bars at $+/-1SD$). Dashed line: error with an OLS fit on the relevant features.

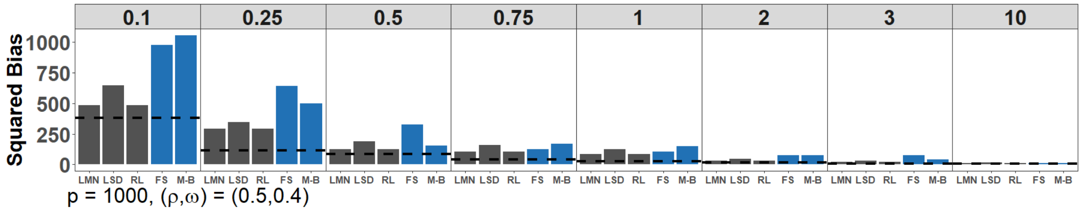


**(c)** Squared bias of $\hat{\beta}$ over simulation replicates. Dashed line: squared bias with an OLS fit on relevant features.

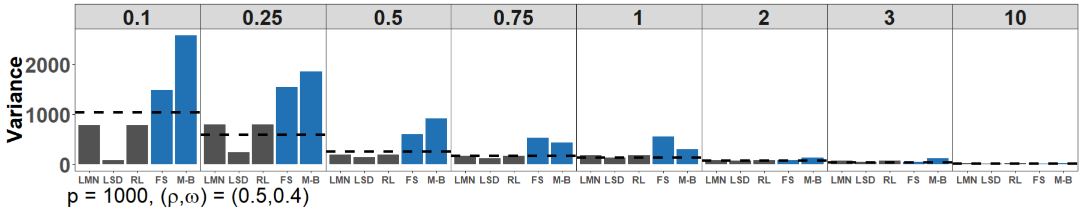


**(d)** Variance of $\hat{\beta}$ over simulation replicates. Dashed line: variance with an OLS fit on relevant features.

**Figure 24:** Summary results in scenarios with $p = 1000$, $k_0 = 10$, various SNR values, and block correlation structure with $(\rho, \omega) = (0.5, 0.4)$. Purple: data whitened using the true covariance (MIP BF, MIP BVR, and FS). Gray: original data.

## 4.5 Sparser scenarios with $p = 100$

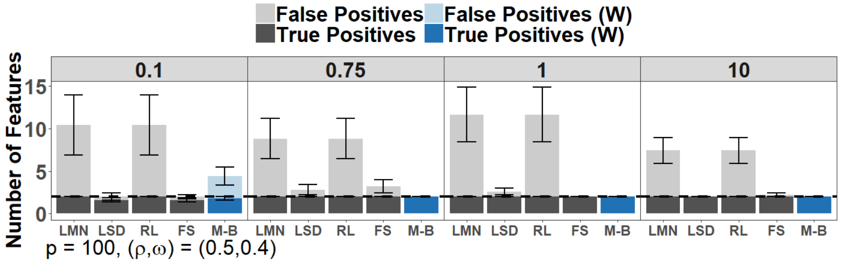


**(a)** Average number of true and false positives over simulation replicates. Bars: $\pm 1SD$, dashed line: $k_o = 2$.

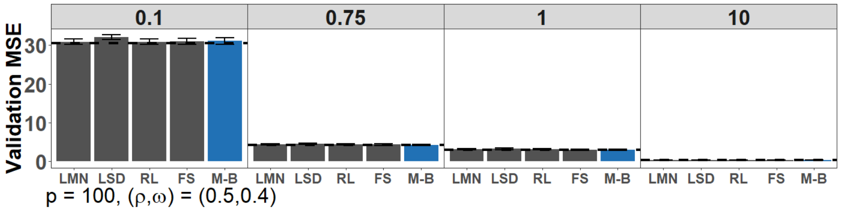


**(b)** Average validation Mean Squared Error over simulation replicates (error bars at $+/-1SD$). Dashed line: error with an OLS fit on the relevant features.

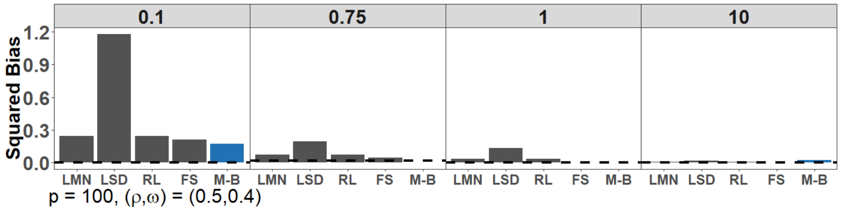


**(c)** Squared bias of $\hat{\beta}$ over simulation replicates. Dashed line: squared bias with an OLS fit on relevant features.

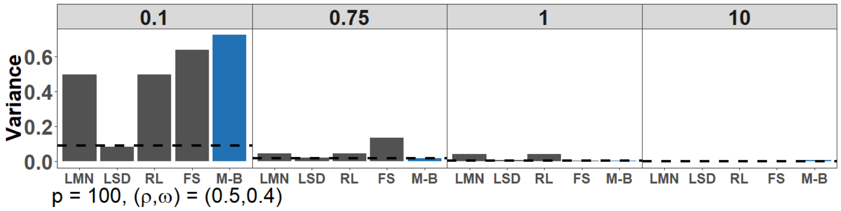


**(d)** Variance of $\hat{\beta}$ over simulation replicates. Dashed line: variance with an OLS fit on relevant features.

**Figure 25:** Summary results in scenarios with $p = 100$, $k_0 = 2$, various SNR values, and block correlation structure with $(\rho, \omega) = (0.5, 0.4)$. Blue: data whitened using the true covariance (MIP BF and MIP BVR). Gray: original data.

# 5 Additional Results for the Computational Burden

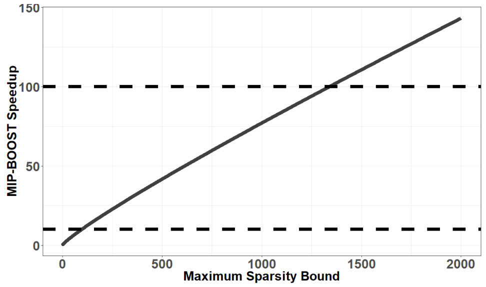


**Figure 26:** Conservative estimate of the MIP-BOOST speedup. Dashed lines: 10x and 100x speedup. Estimate calculated taking the ratio of the total number of bounds explored in traditional cross-validation (the maximum sparsity bound, call it $c$) and the total number under our bisection (at most $log_2(c) + 3$ when the assumptions of our convergence proof in Section 6 are satisfied). Together, it is $\frac{c}{log_2(c)+3}$.

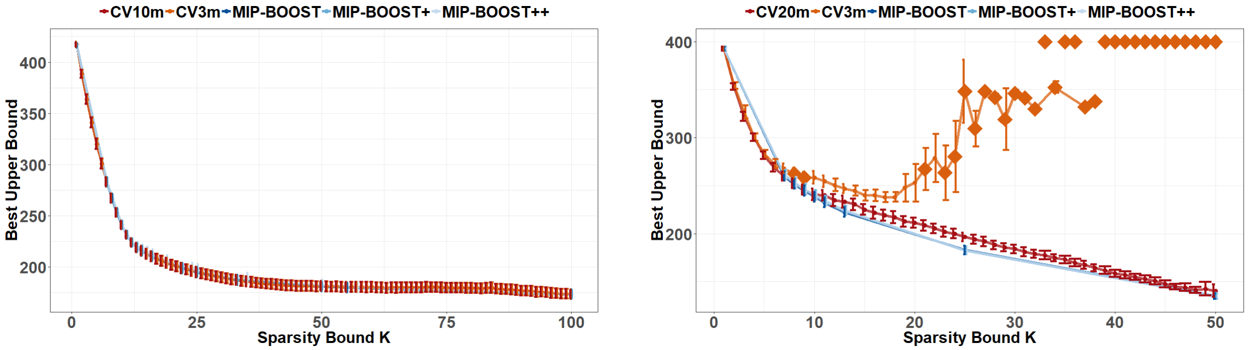


**(a)** Average best upper bound. Bars: $\pm 1SD$.

**(b)** Average best upper bound. Bars: $\pm 1SD$.

**Figure 27:** Summary results of the best upper bound in scenarios with $n = 500$, $p = 100$ (panel (a)); $p = 1000$ (panel (b)); $k_0 = 10$, autoregressive correlations ($\alpha = 0.9$) and $SNR = 1$. Results are averaged over 5 repetitions. $\Diamond$'s denote cases where at least one of the repetitions was unable to find an integer solution within the time limit (successful instances are averaged), and disconnected $\Diamond$'s denote cases with no integer solutions. Upper bound values for MIP-BOOST variants are drawn only for the subset of sparsity bounds visited by the bisection search.

**Table 1:** Percentage of sparsity bounds searched where the average upper bound for a MIP-BOOST variant was equal or stronger than of the naive MIP implementation in standard 10-fold cross-validation

| Procedure | $p = 100$ | | $p = 1000$ | |
|---|---|---|---|---|
| | CV10m | CV3m | CV20m | CV3m |
| MIP-BOOST | 0.75 | 0.81 | 0.96 | 0.98/0.95* |
| MIP-BOOST+ | 0.64 | 0.77 | 0.88 | 0.98/0.95* |
| MIP-BOOST++ | 0.28 | 0.28 | 0.72 | 0.98/0.95* |

*: the percentage only considering the subset of sparsity bounds that produced integer feasible solutions

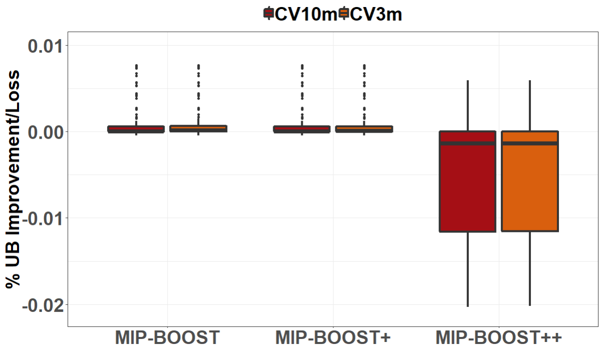


**(a)** Distribution of percentage improvement/loss for $p = 100$ (searched $k = 1, ..., 100$)

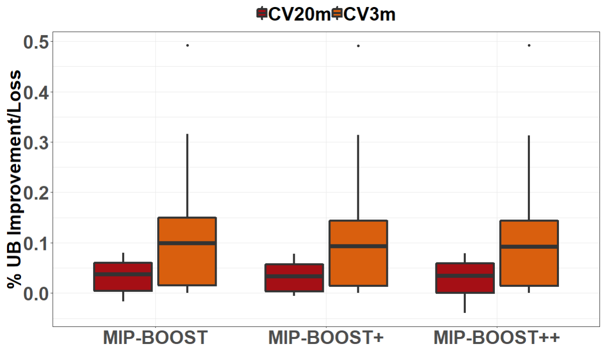


**(b)** Distribution of percentage improvement/loss for $p = 1000$ (searched $k = 1, ..., 50$)

**Figure 28:** Boxplots of the percentage improvement or loss in upper bound over sparsity bounds searched when comparing MIP-BOOST variants to the naive MIP implementation with standard 10-fold cross-validation. For $p = 1000$, only the subset of sparsity bounds where CV3m produced integer solutions are considered when comparing MIP-BOOST variants to CV3m. All $k = 1, .., 50$ are considered when comparing to CV20m, and all $k = 1, ..., 100$ are considered for comparisons on all methods for $p = 100$.

# 6 Bisection with Feelers Convergence Proof Sketch

## Assumptions

To prove convergence of bisection with feelers we assume the following:

1. **Multiple "Elbow" shape:** $\exists x_i^* \in [a_0, c_0]$ (elbows) where $i = 1, ..., l$ such that $\forall i$

   (a) $\exists \tau_i = [x_i^*, x_i^* + \epsilon]$ for some $\epsilon > 0$ such that $x_j^* \notin \tau_i \; \forall j \neq i$

   - Here $\tau_i$ is the non-empty interval representing the "tail" following each elbow with little to no improvement in cross-validation error

   (b) $0 \leq \Delta f(x, y) \leq \delta^*$ for some $\delta^* > 0$ and $\forall x < y$ where $x, y \in \tau_i$

   - Within the tail following each elbow, there is either no change or only minor improvements in cross-validation error.

   (c) $\Delta f(x, y) > \delta^* \; \forall x < y$ where $x$ and $y$ are not both in $\tau_i$

   - Significant improvements between pairs of points as long as both are not in the same tail.

   Note that we have $\Delta f(\cdot, \cdot)$ defined as:

$$\Delta f(x, y) = -\frac{1}{f(x)} \frac{f(y) - f(x)}{(y - x)} \tag{1}$$

2. **Accurate improvement threshold:** $\delta = \delta^*$

We will show that our bisection procedure will converge to $x_l^*$, the elbow with the lowest cross-validation error.

## Proof

We first show that every current interval of our bisection will contain $x_l^*$.
Let $[a_n, c_n]$ denote the $n$th bisection interval and take $n = 0$, the initial interval. By our assumption, $x_l^* \in [a_0, c_0]$ and so $x_l^* \in [a_0, b_0]$ where $b_0 = floor((a_0 + c_0)/2)$ or $x_l^* \in (b_0, c_0]$. If $x_l^* \in [a_0, b_0]$ and $x^* \neq a_0$, then $\Delta f(a_0, b_0) > \delta^*$ since $a_0 \notin \tau_l$ and $b_0 \in \tau_l$.

Also, $\Delta f(b_0, c_0) \leq \delta^*$ since $b_0, c_0 \in \tau_l$.

$\Rightarrow$ we search $[a_1, c_1] = [a_0, b_0]$ next.

If $x_l^* = a_0$, then $\Delta f(a_0, b_0) \leq \delta^*$ and $\Delta f(b_0, c_0) \leq \delta^*$ $(a_0, b_0, c_0 \in \tau_l)$ and we again search $[a_1, c_1] = [a_0, b_0]$.

If $x_l^* \in (b_0, c_0]$, then $\Delta f(b_0, c_0) > \delta^*$ $(b_0 \notin \tau_l,\ c_0 \in \tau_l)$. Additionally, $\Delta f(a_0, b_0) > \delta^*$ or $0 \leq \Delta f(a_0, b_0) \leq \delta^*$ by assumptions.

$\Rightarrow$ we search $[a_1, c_1] = [b_0, c_0]$ next.

In either scenario, $x_l^* \in [a_1, c_1]$.

Now assume this holds for $n = k$ and $x_l^* \in [a_k, c_k]$, then we again have that $x_l^* \in [a_k, b_k]$ or $x_l^* \in (b_k, c_k]$. By the same argument as above if $x_l^* \in [a_k, b_k]$, then we search $[a_{k+1}, c_{k+1}] = [a_k, b_k]$. Also if $x_l^* \in (b_k, c_k]$, then we search $[a_{k+1}, c_{k+1}] = [b_k, c_k]$. In either scenario $x_l^* \in [a_{k+1}, c_{k+1}]$.

Now we have that $x_l^* \in [a_N, c_N]$, our final interval, so $x_l^* = a_N, b_N$, or $c_N$.

If $x_l^* = a_N$, then $\Delta f(a_N, b_N) \leq \delta^*$ and $\Delta f(b_N, c_N) \leq \delta^*$ $(a_N, b_N, c_N \in \tau_l)$.

$\Rightarrow$ our procedure would take $\hat{k}_0 = a_N$.

Similarly, if $x_l^* = b_N$, then $\Delta f(a_N, b_N) > \delta^*$ and $\Delta f(b_N, c_N) \leq \delta^*$ ($a_N \notin \tau_l$ and $b_N, c_N \in \tau_l$).

$\Rightarrow$ our procedure would take $\hat{k}_0 = b_N$.

Finally, if $x_l^* = c_N$, then $\Delta f(a_N, b_N) > \delta^*$ or $0 \leq \Delta f(a_N, b_N) \leq \delta^*$ and $\Delta f(b_N, c_N) > \delta^*$ ($a_N, b_N \notin \tau_l$ and $c_N \in \tau_l$).

$\Rightarrow$ our procedure would take $\hat{k}_0 = c_N$.

In all cases, we converge to $x_l^*$ and have proven convergence of bisection with feelers to the "elbow" with the lowest cross-validation error.

Finally, we note that we proved convergence without the use of "feelers" – and under assumptions on the shape of the CVMSE curve (decreasing with multiple elbows). In practice, we utilize the "feelers" portion to account for fluctuations around this shape, which can occurr when the data contains more noise. In short, our bisection is constructed so that if we do see an increase in the CVMSE curve, we favor sparsity and shift towards a point that still maintains significant improvements ($> \delta^*$) to the left of this increase. However, provided the search length of the feelers ($l_f$) is large enough, we will find that the curve starts to decrease again and follow this improvement as we re-start.

# References


Bertsimas, D., King, A., Mazumder, R. et al. (2016), ‘Best subset selection via a modern optimization lens’, *The Annals of Statistics* **44**(2), 813–852.

Bertsimas, D. & Van Parys, B. (2017), ‘Sparse high-dimensional regression: Exact scalable algorithms and phase transitions’, *arXiv preprint arXiv:1709.10029* .

Hastie, T., Tibshirani, R. & Tibshirani, R. J. (2017), ‘Extended comparisons of best subset selection, forward stepwise selection, and the lasso’, *arXiv preprint arXiv:1707.08692* .
